# Supplementary material for: On the reservoir of sulphur in dark clouds : chemistry and elemental abundance reconciled
Source: arXiv:1704.01404 ancillary file (2017-04-05)
Supplement: Supplementary file 1 [file Supplementary_material__online_.pdf]

MNRAS **000**, 1–30 (2016) Preprint 31 March 2017 Compiled using MNRAS LaTeX style file v3.0

# Appendixes to: On the reservoir of sulphur in dark clouds : chemistry and elemental abundance reconciled

Thomas H. G. Vidal,[1] Jean-Christophe Loison[2,3], Adam Yassin Jaziri[1], Maxime Ruaud[1], Pierre Gratier[1] and Valentine Wakelam[1]
[1]Laboratoire d'astrophysique de Bordeaux, Univ. Bordeaux, CNRS, B18N, allée Geoffroy Saint-Hilaire, 33615 Pessac, France
[2]Univ. Bordeaux, ISM, UMR 5255, F-33400, Talence, France
[3]CNRS, ISM, UMR 5255, F-33400, Talence, France

31 March 2017

## APPENDIX A: RATE CONSTANT AND PRODUCTS DETERMINATION

### A1 General methodology

A large part of the reactions treated in this study have unknown reaction rates (without experimental measurements and/or theoretical calculations to rely upon) in the temperature range of interest (T in the 10-200 K range). To make a reasonable estimate of their reaction rates at low temperature, we first always estimate the presence or not of a barrier through general considerations from a methodology described in Loison et al. (2014) assuming that when the ground state of the adduct (complex) arises from the pairing up of electrons on the two radical reactants then there is no barrier over the Potential Energy Surface (PES), whereas if all the electrons remain unpaired then the surface is likely be repulsive (Smith 2011). Carbon atom reactivity is a special case as carbon atoms react with unsaturated closed shell molecules. We also use the scattered experimental and theoretical studies of similar reactions found through an extensive literature search, and in some critical cases, we performed ab-initio calculations when the general considerations lead to ambiguous results (H, O + carbene reactions for example). In the gas phase, as the temperature is very low (near 10 K) in dense interstellar clouds, we consider only exothermic reactions without a barrier along the reaction coordinate (Smith 2006; Smith 2011), even if some exceptions might exist which can occur through tunneling such as F + $H_2$ (Neufeld et al. 2005) and OH + methanol (Shannon et al. 2013) and C + H2O (Hickson et al. 2016). On grains, H atom addition reactions on unsaturated closed shell molecules present a barrier but may be important as tunneling is often efficient due to the much longer interaction time (Ruaud et al. 2016; Hama & Watanabe 2013).

To estimate the presence (and the value) of a barrier for the critical reactions for which general considerations cannot lead to clear estimate, we performed theoretical calculations. In these cases, we systematically performed DFT calculations using the M06-2X functional with the cc-pVTZ basis set. This highly nonlocal functional developed by Zhao & Truhlar (2008) is well suited for structures and energetics of the transition states. However, as in general the M06-2X functional slightly underestimates barriers (Zhao & Truhlar 2008; Korth & Grimme 2009), we performed MP2 calculations at the cc-pVTZ level and at the CCSD(T) level when the DFT calculations were found to lead to ambiguous results (for example when DFT leads to a submerged barrier, with a TS energy below but close to the entrance level which may happen when there is a van der Waals complex between the reactants (Georgievskii & Klippenstein 2007). When there is no barrier at the MP2 level we consider that the reaction is barrierless as this method usually overestimates barriers (up to several tens of kJ/mol for small barriers) and we applied capture rate theory to calculate the rate constant at low temperature (Loison et al. 2014; Georgievskii & Klippenstein 2005). When there is a barrier at the M06-2X level we consider that there is a notable barrier as this method slightly underestimates barriers (a few kJ/mol for large barriers and as much as 10 kJ/mol for small barriers from our various calculations). In that case we either neglect this reaction or we calculate the rate constant using Transition State Theory (Benson 1976). All ab initio calculations were performed with Gaussian09.

### A2 Branching ratios estimation

Most of the reactions present in the chemical network are addition-elimination reactions. Branching ratios are then controlled by the evolution of the addition complex (which are often a stable molecule). In this study we did not perform RRKM calculations to determine the branching ratios. We estimate the branching ratio by favoring the lower exit transition state coming from the complex as calculated through theoretical calculations and literature review (see references in the Table in appendix B). In the absence of exit transition states, the most exothermic products are considered to have the larger branching ratio as indicated by statistical theory (Galland et al. 2003, 2001; Chabot et al. 2010). When there is one exit channel with much larger exothermicity we only consider that one. When the exothermicities are comparable, we use branching ratio proportional to the exothermicites. To determine the thermochemistry we use Baulch et al. (2005). If the enthalpies of formation were unknown, we performed DFT calculations with the hybrid M06-2X functional. We note that branching ratios are often, but not always, subject to large uncertainties.

© 2016 The Authors

### A3 Electronic Dissociative Recombination

For electronic Dissociative Recombination (DR) reactions, we estimate the rate constant from capture theory as well as from similar reactions (Florescu-Mitchell & Mitchell 2006; Fournier et al. 2013). The size dependency of the DR rate constant is deduced from Fournier et al. (2013) and also Reiter & Janev (2010). For the DR branching ratio we consider that H elimination should be between a few percent and 50%, depending on the number of H atoms of the ions (Florescu-Mitchell & Mitchell 2006; Plessis et al. 2012; Reiter & Janev 2010), with H atom production being always favored versus $H_2$ production (Plessis et al. 2012; Reiter & Janev 2010). As DR reactions are highly exothermic processes, the products may carry a large internal energy ($E_{int}$) leading to isomerization and secondary dissociation. We consider that the internal energy distribution leads to highly excited polyatomic products, similar to the case of the DR of $HNCH^+$ (Mendes et al. 2012). If the internal energy is above the dissociation limit, it will lead to dissociation and if the internal energy is above the isomerization barrier (for HNCS → HSCN for example), it will lead to the production of other isomers whose branching fraction is proportional to the ro-vibrational densities of states of each isomer at the TS energy (Herbst et al. 2000). The ro-vibrational densities of states is calculated using the MESMER program. It should be noted that the branching ratios of DR reactions are often highly uncertain and may in some case be critical for closed shell species ($H_2CS$, $C_3S$) showing low reactivity with atoms (H, N, C, O, S).

### A4 Surface chemistry update

The surface reactions are based on the Langmuir-Hinshelwood mechanism using the formalism of Hasegawa et al. (1992). The network has been updated since through various contributions, among them those of Garrod & Herbst (2006) and Garrod et al. (2007). In the current version of the code, all species diffuse on the surfaces by thermal hopping only. At 10 K, hydrogen atom can efficiently thermally diffuse on the surface. Then to complete the sulphur surface chemical network we consider systematically hydrogen atom reactions, either through addition on unsaturated species or through H atom abstraction (such as s-H + s-$H_2$S → s-$H_2$ + s-HS reaction, 's-' meaning surface species). For all H atom reactions with radicals or with molecules, we use the same activation barrier as in the gas phase, which is indeed a rough approximation. However, the new formalism described in Ruaud et al. (2016), including the competition between diffusion and reaction, increases notably the efficiency of surface reactions with low and medium activation energies through tunneling, and the precise values of the activation energy is not critical as long as tunneling is efficient. We check this effect using the s-H + s-$H_2$S → s-$H_2$ + s-HS reaction by applying either the Kurylo et al. (1971) value of the activation energy (860 K) and the Peng et al. (1999) value equal to 1350 K, both of which lead to very similar results. We used the Tielens & Hagen (1982) adsorption energies for N and O atoms, which allow these atoms to diffuse on the surface. Then we also consider the reactions of oxygen and nitrogen atoms with the various radicals present on the surface (the atom + radical reactions occur without a barrier). We did not consider however the reactions of oxygen and nitrogen atoms with molecules as they show large barriers in the gas phase and for which tunneling is much less efficient than for hydrogen atom reactions. We also consider some minor NH, $NH_2$ and OH reactions involving key species of this study despite the fact that at 10 K they have a low efficiency as NH and $NH_2$ do not diffuse efficiently on ice. In all cases we favor addition channels when they exist, as we consider that the interaction with the surface is efficient enough to redistribute the energy released by bond formation. When the species produced by addition is not stable or with a similar stability to the exit bimolecular channels, we favor the bimolecular products. This is the case for example for the important s-O + s-HCS reaction for which we neglect s-HCOS, s-HSCO and s-HOCS formation using Rice et al. (1993) and Rice & Chabalowski (1994). It should be noted that we neglect the s-CO + s-HS → s-OCS + s-H reaction in contrast to Woods et al. (2015) as this reaction is endothermic by 51 kJ/mol (6134 K) in the gas phase and interaction with ice is unlikely to compensate this exothermicity as HS will be strongly bound to the ice through H-bonding. The efficiency of this reaction may involve complex effects including complexation mechanisms between sulphur atoms and CO on ice. Considering the various uncertainties, the present surface chemistry network for s-$H_2$CS, s-$CH_3$SH, s-OCS, s-HNCS and s-HSCN species is coherent (the s-N + s-HCS reaction is treated below) . However, the networks for s-SO and s-NS are simplified as almost nothing is known on these species so that a considerable amount of work is required for these to be considered. As a result, SO and NS gas phase abundances are controlled by gas phase reactions (which involve high fluxes) and not through grain chemistry (almost no SO and NS desorption at 10 K).

| Species (Energy, hartree) | Relative energies (kJ/mol) | Geometries | Frequencies ($cm^{-1}$) |
|---|---|---|---|
| H (0.4981348) | 0 | | |
| CS (-436.207178) | 0 | C 0.000000 0.000000 -1.111122<br>S 0.000000 0.000000 0.416671 | 1333 |
| 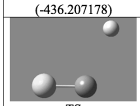 TS (-436.703021) | +6.0 | C 0.093236 1.025058 0.000000<br>S 0.093236 -0.504753 0.000000<br>H -2.051183 1.925697 0.000000 | 187, 1318, 417i |

**Figure A1.** Relative energies at the M06-2X/cc-pVTZ level (in kJ/mol at 0 K including ZPE) with respect to the H + CS energy, geometries and frequencies (in $cm^{-1}$, unscaled, calculated at the M06-2X/cc-pVTZ level) of the various stationary points. The absolute energies at the M06-2X/cc-pVTZ level including ZPE in hartree are also given in column 1.

### A5 Theoretical calculations

#### *A5.1 The H + CS reaction*

We have found a positive barrier for this reaction at the DFT (M06-2X) and MP2 levels for this important grain reaction leading to HCS and being the source of $H_2$CS and $CH_3$SH on grains. Considering the various results, we use a barrier value equal to 1000 K for this reaction, slightly above the M06-2X/cc-pVTZ value (at the M06-2X/cc-pVTZ level of theory the H + CO barrier is calculated equal to 17.1 kJ/mol, slightly below the barrier obtained at a high level of calculations (MRCI+Q/aug-cc-pV6Z) close to 19.0 kJ/mol (Wagner & Bowman 1987; Wang et al. 1973; Peters et al. 2013)).

#### *A5.2 The H + $H_2$CS reaction*

We have found a positive barrier for H atom addition to the carbon and sulphur atoms at the DFT (M06-2X) and MP2 levels (one TS has two imaginary frequencies at the M06-2X level but only one at the MP2 level). Considering the various results, we use barrier values slightly above the M06-2X/cc-pVTZ values. It can be noted that H addition to the sulphur atom is favored versus H atoms addition

**Table A1.** Relative Energies at the MP2/cc-pVTZ level (in kJ/mol at 0 K including ZPE) with respect to the H + CS energy. The absolute energies at the MP2/cc-pVTZ level including ZPE in hartree are also given in column 1.

| Species (energy in hartree) | Relative energies (kJ/mol) |
|---|---|
| H (-0.4998098) | 0 |
| CS (-435.652604) | 0 |
| TS (-436.145404) | +18.4 |

| Species (Energy, hartree) | Relative energies (kJ/mol) | Geometries | Frequencies (cm$^{-1}$) |
|---|---|---|---|
| H (0.4981348) | 0 | | |
| 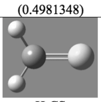<br>$H_2CS$ (-437.429084) | 0 | C -1.018841 0.000000 0.000000<br>H -1.596005 -0.921683 0.000000<br>H -1.596005 0.921683 0.000000<br>S 0.581566 0.000000 0.000000 | 1006, 1053, 1138, 1504, 3094, 3180 |
| 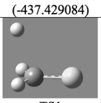<br>TS1 (-437.923736) | +9.1 | S 0.656121 0.050964 0.000000<br>C -0.923195 -0.267941 0.000001<br>H -1.479945 -0.419749 -0.921360<br>H -1.479947 -0.419738 0.921363<br>H -1.998875 1.631708 -0.000005 | 269, 331, 997, 1019, 1082, 1489, 3088, 3176, 604i |
| 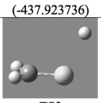<br>TS2 (-437.925373) | +4.8 | C 1.073106 0.149733 0.015580<br>H 1.567236 0.676074 -0.796494<br>H 1.697731 -0.117733 0.863670<br>H -1.864280 1.846367 0.288877<br>S -0.489958 -0.206444 -0.028096 | 134, 1008, 1036, 1107, 1501, 3111, 3202, 409i, 75i |

**Figure A2.** Relative energies at the M06-2X/cc-pVTZ level (in kJ/mol at 0 K including ZPE) with respect to the H + $H_2CS$ energy, geometries and frequencies (in cm$^{-1}$, unscaled, calculated at the M06-2X/cc-pVTZ level) of the various stationary points. The absolute energies at the M06-2X/cc-pVTZ level including ZPE in hartree are also given in column 1.

**Table A2.** Relative Energies at the MP2/cc-pVTZ level (in kJ/mol at 0 K including ZPE) with respect to the H + $H_2CS$ energy. The absolute energies at the MP2/cc-pVTZ level including ZPE in hartree are also given in column 1.

| Species (energy in hartree) | Relative energies (kJ/mol) |
|---|---|
| H (-0.4998098) | 0 |
| $H_2CS$ (-436.866619) | 0 |
| TS1 (-437.347034) | +50.9 |
| TS2 (-437.348263) | +47.7 |

to the carbon atom in contrast to the H + $H_2CO$ case (Hippler & Viskolcz 2002; Oehlers et al. 2000), associated with much lower barrier values.

### *A5.3 The H + $C_3S$ reaction*

We looked for H atom addition to all potential sites. The most favorable addition is on the terminal carbon atom which is logical as this atoms carries the two carbene electrons (••C=C=C=S) and is the most reactive site. We have found positive barriers for this reaction at the DFT (M06-2X) and MP2 levels. Considering the various results, we consider only TS1 with a barrier value slightly above the M06-2X/cc-pVTZ values.

| Species (Energy, hartree) | Relative energies (kJ/mol) | Geometries | Frequencies (cm$^{-1}$) |
|---|---|---|---|
| H (0.4981348) | 0 | | |
| 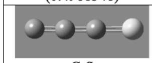<br>$C_3S$ (-512.324228) | 0 | C 0.000000 0.041616 0.000000<br>C 0.282933 1.302727 0.000000<br>C 0.592815 2.535795 0.000000<br>S -0.328406 -1.455052 0.000000 | 146, 508, 508, 754, 1597, 2157 |
| 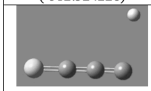<br>TS1 (-512.820744) | +4.2 | S -1.579017 0.057122 -0.000003<br>C -0.051668 -0.066322 0.000005<br>C 1.236387 -0.169750 0.000012<br>C 2.502957 -0.289890 -0.000010<br>C 3.138209 2.241829 0.000000 | 91, 163, 175, 502, 509, 751, 1594, 2156, 246i |
| 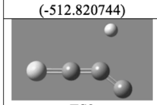<br>TS2 (-512.810812) | +30.3 | S 1.502145 -0.088335 0.000065<br>C 0.033402 0.087614 -0.000310<br>C -1.332796 -0.014921 0.000010<br>C -2.596705 -0.161861 0.000096<br>H -0.256895 1.948373 0.000179 | 178, 185, 319, 518, 520, 754, 1538, 2121, 978i |
| 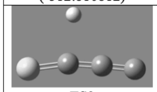<br>TS3 (-512.810510) | +31.1 | S -1.501496 -0.069251 0.000001<br>C 0.020757 0.083776 -0.000006<br>C 1.318004 0.222934 -0.000001<br>C 2.399407 -0.470118 0.000002<br>H 1.594930 2.088460 0.000005 | 175, 210, 311, 489, 509, 817, 1592, 2034, 748i |
| 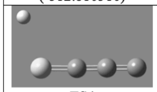<br>TS4 (-512.817544) | +12.7 | S -1.424554 -0.136596 0.000000<br>C 0.109345 -0.066449 0.000001<br>C 1.397973 0.013812 0.000002<br>C 2.669367 0.083915 -0.000001<br>H -2.267242 1.997873 0.000000 | 159, 165, 257, 494, 506, 745, 1583, 2144, 541i |

**Figure A3.** Relative energies at the M06-2X/cc-pVTZ level (in kJ/mol at 0 K including ZPE) with respect to the H + $C_3S$ energy, geometries and frequencies (in cm$^{-1}$, unscaled, calculated at the M06-2X/cc-pVTZ level) of the various stationary points. The absolute energies at the M06-2X/cc-pVTZ level including ZPE in hartree are also given in column 1.

**Table A3.** Relative Energies at the MP2/cc-pVTZ level (in kJ/mol at 0 K including ZPE) with respect to the H + $C_3S$ energy. The absolute energies at the MP2/cc-pVTZ level including ZPE in hartree are also given in column 1.

| Species (energy in hartree) | Relative energies (kJ/mol) |
|---|---|
| H (-0.4998098) | 0 |
| $C_3S$ (-511.611590) | 0 |
| TS1 (-512.101631) | +25.6 |

### *A5.4 The H + HNCS reaction*

This reaction plays a role only for grains chemistry only as for any H + closed shell molecules there is a barrier for addition on any sites (N, C or S). We have found large positive barriers for H addition on N, C and S atoms at DFT (M06-2X) level. As the M06-2X/cc-pVTZ calculations lead to relatively high values which is in general associated to relatively low uncertainties, we use barrier values slightly above the M06-2X/cc-pVTZ values.

### *A5.5 The H + HSCN reaction*

This reaction plays a role only for grains chemistry only as for any H + closed shell molecules there is a barrier for addition on any sites (N, C or S). We have found large positive barriers for H addition on N and C atoms at DFT (M06-2X) level. The addition to sulphur atom is not possible as it leads only to $H_2S$ + CN product which is an endothermic exit channel. As the M06-2X/cc-pVTZ calculations lead to relatively high values which is in general associated to relatively low uncertainties, we use barrier values slightly above the

| Species (Energy, hartree) | Relative energies (kJ/mol) | Geometries | Frequencies ($cm^{-1}$) |
|---|---|---|---|
| H<br>(0.4981348) | 0 | | |
| 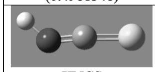<br>HNCS<br>(-491.615021) | 0 | C 0.495921 0.006919 -0.000008<br>S -1.075582 0.008336 0.000001<br>N 1.683282 -0.102642 0.000003<br>H 2.450808 0.543611 0.000005 | 436, 498, 566, 887, 2094, 3723 |
| 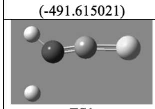<br>TS1<br>(-492.102291) | +28.5 | N -1.607473 -0.063572 -0.000069<br>H -2.321081 -0.769587 0.000332<br>C -0.404382 -0.123403 -0.000035<br>S 1.155350 0.035341 0.000014<br>H -2.485924 1.389554 0.000138 | 211, 324, 504, 596, 816, 910, 2026, 3696, 962i |
| 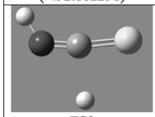<br>TS2<br>(-492.096237) | +44.4 | N -1.702265 -0.015544 -0.000009<br>H -2.216100 -0.885418 0.000051<br>C -0.499824 0.066529 -0.000003<br>S 1.090654 -0.077901 0.000000<br>H -0.319568 1.841467 0.000025 | 367, 494, 523, 605, 707, 865, 1999, 3625, 1056i |
| 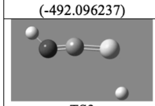<br>TS3<br>(-492.106776) | +16.8 | N 1.733514 0.178120 -0.000132<br>H 2.529924 -0.437216 0.000581<br>C 0.559148 -0.052774 0.000070<br>S -1.014056 -0.141174 -0.000019<br>H -1.794517 1.765809 0.000226 | 225, 244, 440, 484, 644, 876, 2068, 3673 701i |

**Figure A4.** Relative energies at the M06-2X/cc-pVTZ level (in kJ/mol at 0 K including ZPE) with respect to the H + HNCS energy, geometries and frequencies (in $cm^{-1}$, unscaled, calculated at the M06-2X/cc-pVTZ level) of the various stationary points. The absolute energies at the M06-2X/cc-pVTZ level including ZPE in hartree are also given in column 1.

| Species (Energy, hartree) | Relative energies (kJ/mol) | Geometries | Frequencies ($cm^{-1}$) |
|---|---|---|---|
| H<br>(0.4981348) | 0 | | |
| 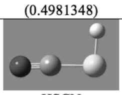<br>HSCN<br>(-491.600573) | 0 | C 0.699105 0.005712 0.000005<br>N 1.848680 0.007482 -0.000002<br>S -0.998201 -0.083468 -0.000001<br>H -1.164171 1.248845 -0.000001 | 349, 407, 713, 984, 2350, 2736 |
| 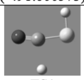<br>TS1<br>(-492.086550) | +31.9 | N 1.816554 -0.200291 -0.000009<br>S -1.026379 0.026321 -0.000029<br>H -1.087005 -1.317520 0.000410<br>C 0.687214 0.069703 -0.000029<br>H 0.669909 1.880200 0.000294 | 335, 430, 442, 541, 721, 985, 2228, 2709, 895i |
| 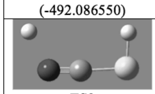<br>TS2<br>(-492.086469) | +32.1 | N 1.761914 -0.155589 -0.000107<br>H 2.521471 1.294173 -0.000141<br>C 0.600423 -0.150986 0.000261<br>S -1.083901 -0.037991 -0.000055<br>H -1.114990 1.308720 0.000206 | 230, 264, 431, 527, 719, 966, 2209, 2692, 1046i |
| 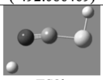<br>TS2b<br>(-492.087260) | +30.1 | N 1.760922 -0.168674 -0.000132<br>H 2.555722 1.276955 0.000939<br>C 0.599259 -0.170634 -0.000039<br>S -1.065812 0.130717 -0.000055<br>H -1.424735 -1.163909 0.001100 | 255, 432, 532, 707, 988, 2208, 2620, 1030i, 111i |
| 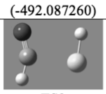<br>TS3<br>(-492.127064) | -74.4 | N 1.636357 -0.501286 -0.076068<br>S -1.110746 -0.010587 -0.064407<br>H 0.963508 -0.878246 0.945303<br>C 1.045149 0.499632 0.064593<br>H 1.010045 1.558843 0.230132 | 93, 283, 646, 758, 838, 1993, 2742, 3328, 448i |

**Figure A5.** Relative energies at the M06-2X/cc-pVTZ level (in kJ/mol at 0 K including ZPE) with respect to the H + HSCN energy, geometries and frequencies (in $cm^{-1}$, unscaled, calculated at the M06-2X/cc-pVTZ level) of the various stationary points. The absolute energies at the M06-2X/cc-pVTZ level including ZPE in hartree are also given in column 1.

M06-2X/cc-pVTZ values. The HSCHN formation is exothermic by -108 kJ/mol and the HCN + SH exit channel by -103 kJ/mol with a TS located at -74.4 kJ/mol below the H + HSCN entrance channel. Then some HCN + SH will likely be produced.

| Species (Energy, hartree) | Relative energies (kJ/mol) | Geometries | Frequencies ($cm^{-1}$) |
|---|---|---|---|
| NH<br>(-55.208739) | 0 | N 0.000000 0.000000 0.129600<br>H 0.000000 0.000000 -0.907200 | 3237 |
| CS<br>(-436.207178) | 0 | C 0.000000 0.000000 -1.111122<br>S 0.000000 0.000000 0.416671 | 1333 |
| 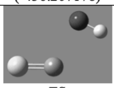<br>TS<br>(-491.415414) | +1.3 | C -0.126285 0.707571 -0.000202<br>S 1.138102 -0.156638 0.000058<br>N -2.116802 -0.329367 -0.000135<br>H -2.634312 0.566362 0.001221 | 119, 184, 610, 1326, 3307, 333i |
| 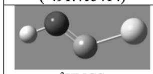<br>$^3$HNCS<br>(-491.504512) | -232.6 | C 0.588397 0.490614 -0.021255<br>S -1.055472 -0.066774 0.007738<br>N 1.553529 -0.276146 -0.030217<br>H 2.482464 0.057724 0.215239 | 297, 481, 714, 932, 1705, 3496 |

**Figure A6.** Relative energies at the M06-2X/cc-pVTZ level (in kJ/mol at 0 K including ZPE) with respect to the CS + NH energy, geometries and frequencies (in $cm^{-1}$, unscaled, calculated at the M06-2X/cc-pVTZ level) of the various stationary points. The absolute energies at the M06-2X/cc-pVTZ level including ZPE in hartree are also given in column 1.

**Table A4.** Relative Energies at the MP2/cc-pVTZ level (in kJ/mol at 0 K including ZPE) with respect to the CS + NH energy. The absolute energies at the MP2/cc-pVTZ level including ZPE in hartree are also given in column 1.

| Species (energy in hartree) | Relative energies (kJ/mol) |
|---|---|
| NH (-55.110246) | 0 |
| CS (-435.652604) | 0 |
| TS (-490.749731) | +34.4 |

### *A5.6 The CS + NH reaction*

We have found a positive barrier for this reaction at the DFT and MP2 levels for the first step of this reaction which is HNCS formation in its excited triplet state (NH has a ground triplet state). There is very little doubt that this reaction has a barrier in the entrance valley as DFT leads to a barrier. We estimate the rate constant using TST theory. Branching ratios are controlled by the evolution of the HNCS adduct. The two possible exit channel are H + NCS and HNC + S. The H + NCS reaction has no TS on the exit channel (radical-radical pathway) and the S + HNC is likely to have a small TS (much below the CN + NH entrance channel) in the exit channel. Considering the exothermicities (H + NCS ΔHr = -147 kJ/mol and S + HNC ΔHr = -187 kJ/mol) we favor S + HNC production.

### *A5.7 The CS + $NH_2$ reaction*

This reaction is potentially very important for HNCS formation. We have found a submerged barrier at the DFT level and a positive barrier at the MP2 and CCD(T) levels for the for the first step of this reaction which is H2NCS formation in it ground state. We consider then that this reaction has a barrier in the entrance valley and is negligible at low temperature in the gas phase. We estimate the rate constant using TST theory with entropy variation calculated at MP2 level and barrier energy at CCSD(T) level. The most favorable exit channel is H + HNCS in gas phase and NH2CS on grain.

### *A5.8 The CS + $C_2H_3$ reaction*

This is not a very important reaction for interstellar cloud chemistry but may be an important one for Titan's atmosphere (Hickson et al. 2014). We have found no barrier at the DFT level and a positive

| Species<br>(Energy, hartree) | Relative energies<br>(kJ/mol) | Geometries | Frequencies<br>($cm^{-1}$) |
|---|---|---|---|
| $NH_2$<br>(-55.849961) | 0 | N 0.000000 0.000000 0.141743<br>H 0.000000 0.802406 -0.496100<br>H 0.000000 -0.802406 -0.496100 | 1534, 3393,<br>3487 |
| CS<br>(-436.207178) | 0 | C 0.000000 0.000000 -1.111122<br>S 0.000000 0.000000 0.416671 | 1333 |
| 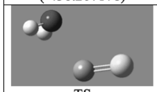<br>TS<br>(-492.058060) | -2.4 | C -0.011760 0.717135 0.000135<br>S 1.237469 -0.166087 -0.000037<br>N -2.124086 -0.307842 -0.000190<br>H -2.429773 0.253880 0.799881<br>H 2.430565 0.255603 -0.798765 | 157, 165,<br>475, 567,<br>1339, 1549,<br>3413, 3506,<br>230i |

**Figure A7.** Relative energies at the M06-2X/cc-pVTZ level (in kJ/mol at 0 K including ZPE) with respect to the CS + $NH_2$ energy, geometries and frequencies (in $cm^{-1}$, unscaled, calculated at the M06-2X/cc-pVTZ level) of the various stationary points. The absolute energies at the M06-2X/cc-pVTZ level including ZPE in hartree are also given in column 1.

**Table A5.** Relative energies (in kJ/mol at 0 K including ZPE) with respect to the CS + $NH_2$ energy at the MP2/cc-pVTZ level. The absolute energies at the MP2/cc-pVTZ level including ZPE in hartree are also given in column 1.

| Species (energy in hartree) | Relative energies (kJ/mol) |
|---|---|
| $NH_2$ (-55.751100) | 0 |
| CS (-435.652604) | 0 |
| TS (-491.397561) | +16.1 |

**Table A6.** Relative energies at the CCSD(T)/cc-pVTZ level (in kJ/mol at 0 K with ZPE calculated at MP2/cc-pVTZ level) with respect to the CS + $NH_2$ energy, the geometries being calculated at the MP2/cc-pVTZ level. The absolute energies at CCSD(T)/cc-pVTZ level without ZPE in hartree are also given in column 1, as well as the ZPE calculated at MP2/cc-pVTZ level.

| Species (energy + ZPE in hartree) | Relative energies (kJ/mol) |
|---|---|
| $NH_2$ (-55.7935892 + 0.019489) | 0 |
| CS (-435.6927335 + 0.002958) | 0 |
| TS (-491.4882355 + 0.026147) | +4.7 |

**Table A7.** Relative energies at the CCSD(T)/cc-pVQZ level (in kJ/mol at 0 K with ZPE calculated at MP2/cc-pVTZ level) with respect to the CS + $NH_2$ energy, the geometries being calculated at the MP2/cc-pVTZ level. The absolute energies at CCSD(T)/cc-pVQZ level without ZPE in hartree are also given in column 1, as well as the ZPE calculated at MP2/cc-pVTZ level.

| Species (energy + ZPE in hartree) | Relative energies (kJ/mol) |
|---|---|
| $NH_2$ (-55.7935892 + 0.019489) | 0 |
| CS (-435.6927335 + 0.002958) | 0 |
| TS (-491.5331085 + 0.026147) | +3.0 |

barrier at the MP2 and CCSD(T) levels for the for the first step of this reaction which is $C_2H_3CS$ formation (through TS1). Moreover, the production of $H_2C_3S$ + H (through TS2) shows an exit barrier at the MP2 and DFT levels. At the DFT level, we have found a pathway leading to $H_2C_3S$ + H involving isomerization (TS3) from $C_2H_3CS$ to $CH_3CCS$. Considering the positive barrier at the CCSD(T) level, we consider that this reaction has a small barrier in the entrance

| Species<br>(Energy, hartree) | Reamtive energies<br>(kJ/mol) | Geometries | Frequencies<br>($cm^{-1}$) |
|---|---|---|---|
| $C_2H_3$<br>(-77.667348) | 0 | C 0.576527 0.030443 -0.000359<br>C -0.692391 -0.145690 0.000041<br>H 1.004687 1.029193 0.000690<br>H 1.271133 -0.798933 0.000930<br>H -1.580634 0.461221 0.000292 | 734, 987, 1060,<br>1086, 1429,<br>1911, 3140,<br>3240, 3311 |
| CS<br>(-435.652604) | 0 | C 0.000000 0.000000 0.005193<br>S 0.000000 0.000000 1.548875 | 1298 |
| 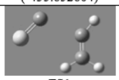<br>TS1<br>(-513.316488) | +9.1 | C 2.030173 -0.652157 0.002001<br>C 1.749570 0.595249 -0.003145<br>H 3.058099 -1.005416 0.000311<br>H 1.253932 -1.409666 0.008374<br>H 2.248005 1.546608 -0.009501<br>C -0.730789 1.000992 0.006173<br>S -1.553360 -0.299752 -0.001835 | 48, 109, 211,<br>233, 706, 1002,<br>1061, 1061,<br>1391, 1432,<br>1938, 3132,<br>3210, 3336<br>268i |
| 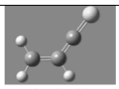<br>$CH_2CHCS$<br>(-513.414440) | -248.1 | C 1.583223 -1.600221 0.000000<br>C 1.234643 -0.265541 0.000000<br>H 2.621285 -1.880271 0.000000<br>H 0.833151 -2.372511 0.000000<br>H 1.997453 0.505443 0.000000<br>C 0.000000 0.241454 0.000000<br>S -1.397443 0.843324 0.000000 | 192, 314, 538,<br>653, 711, 863,<br>896, 1070, 1174,<br>1345, 1509,<br>1855, 3205,<br>3229, 3344 |
| 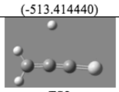<br>TS2<br>(-513.288327) | +83.0 | C -2.460288 -0.158138 -0.000003<br>C -1.115022 -0.044105 -0.000004<br>H -3.093814 0.712608 -0.000130<br>H -2.906852 -1.140390 0.000112<br>H -1.095759 2.423194 0.000089<br>C 0.142445 -0.028222 -0.000001<br>S 1.730851 -0.038289 -0.000002 | 182, 207, 221,<br>282, 446,<br>449, 609, 674,<br>979, 1267, 1452,<br>1745, 3206, 3314<br>291i |
| 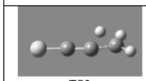<br>TS3<br>(-513.354852) | -91.6 | C 2.456794 0.158835 -0.045835<br>C 1.094275 -0.225472 -0.083312<br>H 3.221114 -0.568783 -0.266260<br>H 2.745590 1.148700 0.280327<br>H 1.628190 -0.623446 0.893717<br>C -0.172530 -0.042006 -0.039933<br>S -1.741633 0.043462 0.006669 | |
| 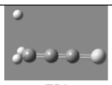<br>TS4<br>(-513.310789) | +24.1 | C -2.340590 -0.213868 0.000004<br>C -1.042581 -0.131085 -0.000001<br>H -2.905509 -0.264565 0.922028<br>H -3.122082 2.129930 -0.000028<br>H -2.905513 -0.264637 -0.922014<br>C 0.206689 -0.050583 0.000000<br>S 1.749500 0.048281 0.000000 | 138, 215, 253,<br>263, 525, 679,<br>725, 1100, 1118,<br>1429, 1606,<br>2202, 3177,<br>3268,<br>253i |
| 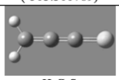<br>$H_2C_3S$<br>(-512.847331) | -71.4 | C 0.000038 0.000000 -0.003025<br>C 0.001797 0.000000 1.321321<br>C 0.003674 0.000000 2.596373<br>S 0.006018 0.000000 4.170595<br>H 0.924646 0.000000 -0.571040<br>H -0.926064 0.000000 -0.568597 | 133, 196, 357,<br>549, 699, 966,<br>1049, 1380,<br>1535, 2104,<br>3131, 3215, |
| H<br>(-0.4998098) | -71.4 | | |

**Figure A8.** Relative energies at the MP2/cc-pVTZ level (in kJ/mol at 0 K including ZPE) with respect to the CS + $C_2H_3$ energy, geometries and frequencies (in $cm^{-1}$, unscaled) of the various stationary points. The absolute energies at the MP2/cc-pVTZ level including ZPE in hartree are also given in column 1.

**Table A8.** Relative energies at the CCSD(T)/cc-pVTZ level (in kJ/mol at 0 K with ZPE) calculated at MP2/cc-pVTZ level) with respect to the CS + $NH_2$ energy, the geometries being calculated at the MP2/cc-pVTZ level. The absolute energies at CCSD(T)/cc-pVTZ level without ZPE in hartree are also given in column 1, as well as the ZPE calculated at MP2/cc-pVTZ level.

| Species (energy + ZPE in hartree) | Relative energies (kJ/mol) |
|---|---|
| $C_2H_3$ (-77.7508239 + 0.038496) | 0 |
| CS (-435.6927335 + 0.002958) | 0 |
| TS (-513.4440054 + 0.042998) | +2.9 |

valley but may have accessible exit channels. We estimate the rate constant using TST theory with entropy variation calculated at the MP2 level and the barrier energy at the CCSD(T) level.

### *A5.9 The O + $C_3S$ reaction*

This is critical reaction for the C3S abundance in molecular clouds as it may be the major $C_3S$ loss process. The most favorable addition is on the terminal carbon atom which is logical as this atoms carries the two carbene electrons (••C=C=C=S) and is the most reactive site. We have found a submerged barrier at the DFT level and relatively large barrier at the MP2 and CCD(T) levels for the first step of this reaction which is OCCCS formation. Considering the

**Table A9.** Relative energies at the M06-2X/cc-pVTZ level (in kJ/mol at 0 K including ZPE) with respect to the CS + $NH_2$ energy. The absolute energies at the M06-2X/cc-pVTZ level including ZPE in hartree are also given in column 1.

| Species (energy in hartree) | Relative energies (kJ/mol) |
|---|---|
| $C_2H_3$ (-77.851299) | 0 |
| CS (-436.207178) | 0 |
| no TS | - |
| $CH_2CHCS$ (-514.161071) | -269.4 |
| TS2 (-514.034685) | +62.5 |
| TS3 (-514.093834) | -92.8 |
| TS4 (-514.068751) | -27.0 |
| $H_2C_3S$ (-513.573158) | -33.6 |
| H (-0.4981348) | -33.6 |

| Species (Energy, hartree) | Relative energies (kJ/mol) | Geometries | Frequencies ($cm^{-1}$) |
|---|---|---|---|
| $C_3S$ (-512.324228) | 0 | C 0.000000 0.041616 0.000000<br>C 0.282933 1.302727 0.000000<br>C 0.592815 2.535795 0.000000<br>S -0.328406 -1.455052 0.000000 | 146, 508, 508, 754, 1597, 2157 |
| O (-75.0642417) | 0 | | |
| 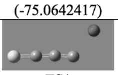 TS1 (-587.391411) | -7.7 | S -1.371612 -1.824494 0.000000<br>C -0.625036 -0.487954 0.000000<br>C 0.000000 0.643880 0.000000<br>C 0.543931 1.789771 0.000000<br>O 2.804053 2.189715 0.000000 | 55, 151, 191, 499, 508, 753, 1064, 2162, 156i |

**Figure A9.** Relative energies at the M06-2X/cc-pVTZ level (in kJ/mol at 0 K including ZPE) with respect to the O + $C_3S$ energy, geometries and frequencies (in $cm^{-1}$, unscaled) of the various stationary points. The absolute energies at the M06-2X/cc-pVTZ level including ZPE in hartree are also given in column 1.

**Table A10.** Relative energies (in kJ/mol at 0 K including ZPE) with respect to the O + $C_3S$ energy at the MP2/cc-pVTZ level. The absolute energies at the MP2/cc-pVTZ level including ZPE in hartree are also given in column 1.

| Species (energy in hartree) | Relative energies (kJ/mol) |
|---|---|
| $C_3S$ (-511.611590) | 0 |
| O (-74.9549023) | 0 |
| TS1 (-586.556252) | +26.9 |

value of the barrier at the CCSD(T) level, we assume this reaction has a barrier in the entrance valley. The rate constant expression in KIDA, for which the origin is unknown, seems a reasonable value and we decided not to change it. It should be noted that there are large uncertainties in the activation energy, and also that tunneling may lead to substantial rate constant value at low temperature as for the O + propene reaction (Sabbah et al. 2007) which also shows a small barrier in the entrance valley. The most favorable products are CO + $C_2S$ in the gas phase.

### *A5.10 The O + HCNS reaction*

We found large barriers for O atom addition to the C and S atoms at the MP2 and CCSD levels, but no barriers at the M06-2X level. The energies at the M06-2X level of the geometries corresponding to TS1 and TS2 at the MP2 level are found to be well below the

**Table A11.** Relative energies at the CCSD(T)/cc-pVTZ level (in kJ/mol at 0 K with ZPE calculated at MP2/cc-pVTZ level) with respect to the O + $C_3S$ energy, the geometries being calculated at the MP2/cc-pVTZ level. The absolute energies at CCSD(T)/cc-pVTZ level without ZPE in hartree are also given in column 1, as well as the ZPE calculated at MP2/cc-pVTZ level.

| Species (energy + ZPE in hartree) | Relative energies (kJ/mol) |
|---|---|
| $C_3S$ (-511.6749015 + 0.012856) | 0 |
| O (-74.9739618) | 0 |
| TS1 (-586.6468614 + 0.014765) | +10.3 |

| Species (Energy, hartree) | Relative energies (kJ/mol) | Geometries | Frequencies ($cm^{-1}$) |
|---|---|---|---|
| O (-74.9549023) | 0 | | |
| 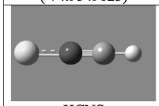 HCNS (-490.912039) | 0 | S 0.000000 0.000000 1.051548<br>C 0.000000 0.000000 -1.716940<br>N 0.000000 0.000000 -0.534999<br>H 0.000000 0.000000 -2.778139 | 74, 74, 431, 431, 799, 1946, 3491 |
| 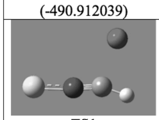 TS1 (-565.835253) | +83.3 | S -1.559990 -0.235929 -0.000062<br>C 0.955510 0.824443 -0.000464<br>N -0.113067 0.423383 0.000430<br>H 1.743132 1.539342 0.000593<br>O 2.284389 -0.709353 0.000022 | 132, 472, 495, 695, 778, 883, 2519, 3533, 984i |
| 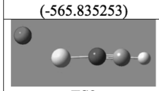 TS2 (-565.844383) | +59.2 | S 0.433146 -0.323602 0.000003<br>C -2.352724 0.227991 -0.000003<br>N -1.223261 0.057741 -0.000016<br>H -3.405482 0.379025 0.000064<br>O 2.394290 0.378309 0.000001 | 116, 360, 418, 493, 691, 797, 3193, 4065, 505i |

**Figure A10.** Relative energies at the MP2/cc-pVTZ level (in kJ/mol at 0 K including ZPE) with respect to the O + HCNS energy, geometries and frequencies (in $cm^{-1}$, unscaled) of the various stationary points. The absolute energies at the MP2/cc-pVTZ level including ZPE in hartree are also given in column 1.

entrance valley. It should be noted that the structure of the HCNS species shows a short CN bond corresponding to a triple bond and then to an hyper-valent N atom. The geometries found at the MP2 and M06-2X levels are in good agreement with previous calculations (Wierzejewska & Moc 2003). The large differences between the three calculations make it difficult to estimate the rate constant for this reaction. Clearly more calculations taking into account the potential multiconfigurational aspect of wavefunctions describing this reaction (use of the multireference configuration interaction method (MRCI) method is required which is beyond the scope of this article). Considering the hyper-valent aspect of the CN bond, we assume that the MP2 and CCSD(T) methods overestimate (significantly) the barrier and we consider no barrier for this reaction leading to both SO + HCN and HCO + NS as products in equal proportion. The uncertainties are very large for this reaction.

### *A5.11 S + c-$C_3H_3^+$ reaction*

We have found a submerged barrier for S addition to c-$C_3H_3^+$ at the M06-2X and MP2 levels. Then, there is little doubt that this reaction has a high rate constant at low temperature even if the rate constant temperature dependence may be relatively complex. We have also performed M06-2X/cc-pVTZ calculations on the O + c-$C_3H_3^+$ reaction which show a barrier of +29.6 kJ/mol, in good agreement with experimental work which found that reaction does

**Table A12.** Relative energies at the CCSD(T)/cc-pVTZ level (in kJ/mol at 0 K with ZPE) calculated at MP2/cc-pVTZ level) with respect to the O + HCNS energy, the geometries being calculated at the MP2/cc-pVTZ level. The absolute energies at CCSD(T)/cc-pVTZ level without ZPE in hartree are also given in column 1, as well as the ZPE calculated at MP2/cc-pVTZ level.

| Species (energy + ZPE in hartree) | Relative energies (kJ/mol) |
|---|---|
| O (-74.9739618) | 0 |
| HCNS (-490.9677888 + 0.016508) | 0 |
| TS1 (-565.9391699 + 0.021659) | +20.2 |
| TS2 (-565.9411838 + 0.023090) | +18.8 |

**Table A13.** Relative energies at the M06-2X/cc-pVTZ level (in kJ/mol at 0 K including ZPE) with respect to the O + HCNS energy, the TS geometries being fixed at the MP2/cc-pVTZ one. The absolute energies at the M06-2X/cc-pVTZ level including ZPE in hartree are also given in column 1.

| Species (energy in hartree) | Relative energies (kJ/mol) |
|---|---|
| O (-75.0642417) | 0 |
| HCNS (-491.558958) | 0 |
| TS1 (MP2 geometry) (-566.630029) | -17.9 |
| TS2 (MP2 geometry) (-566.628446) | -13.8 |

| Species (Energy, hartree) | Relative energies (kJ/mol) | Geometries | Frequencies ($cm^{-1}$) |
|---|---|---|---|
| S (-398.1012399) | 0 | | |
| 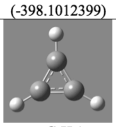 $c-C_3H_3^+$ (-115.676600) | 0 | C -0.780708 -0.058794 -0.000112<br>C 0.339383 0.705313 0.000040<br>C 0.441243 -0.646582 0.000040<br>H -1.857787 -0.139958 0.000320<br>H 0.807850 1.678892 -0.000062<br>H 1.050427 -1.538557 -0.000063 | 778, 946, 954, 1028, 1047, 1054, 1350, 1350, 1692, 3249, 3264, 3314 |
| 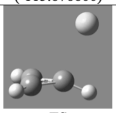 TS (-513.781509) | -9.6 | C 0.647737 -0.000177 0.667216<br>C 1.491987 -0.663051 -0.222279<br>C 1.491833 0.663227 -0.222001<br>H 0.331273 -0.000627 1.695684<br>H 1.887718 -1.598365 -0.583256<br>H 1.887343 1.598813 -0.582513<br>S -1.618480 0.000012 -0.116721 | 170, 203, 806, 928, 964, 1011, 1034, 1958, 1248, 1290, 1673, 3278, 3287, 3332, 189i |

**Figure A11.** Relative energies at the M06-2X/cc-pVTZ level (in kJ/mol at 0 K including ZPE) with respect to the S + $c-C_3H_3^+$ energy, geometries and frequencies (in $cm^{-1}$, unscaled) of the various stationary points. The absolute energies at the M06-2X/cc-pVTZ level including ZPE in hartree are also given in column 1.

not occur (Scott et al. 2000). Considering the higher reactivity of the linear isomer $l-C_3H_3^+$, which reacts with N (Scott et al. 1999) and O (Scott et al. 2000) atoms in contrast to $c-C_3H_3^+$, we consider that $l-C_3H_3^+$ reacts with S atoms and we use a rate constant equal to half the value given by capture rate theory by comparison with O + $l-C_3H_3^+$ reaction. Product branching ratios are deduced from the potential evolution of the $SC_3H_3^+$ intermediate formed in the first step of the reaction. The branching ratios are not highly critical in that case as long as the $HC_3S^+/H_2C_3S^+$ production is not negligible. We consider a branching ratio of 20% for S + $c,l-C_3H_3^+$ → $H_2$ + $HC_3S^+$ and 40% for S + $l-C_3H_3^+$ → H + $H_2C_3S^+$ from the exothermicities.

**Table A14.** Relative energies (in kJ/mol at 0 K including ZPE) with respect to the S + $c-C_3H_3^+$ energy at the MP2/cc-pVTZ level. The absolute energies at the MP2/cc-pVTZ level including ZPE in hartree are also given in column 1.

| Species (energy in hartree) | Relative energies (kJ/mol) |
|---|---|
| S (-397.6258023) | 0 |
| $c-C_3H_3^+$ (-115.422264) | 0 |
| TS (-513.049365) | -3.4 |

**Table A15.** Relative energies (in kJ/mol at 0 K including ZPE) with respect to the N + HCS energy at the MP2/aug-cc-pVTZ level.

| Products of the N + HCS reaction | ΔHr (kJ/mol) |
|---|---|
| HNCS | -637 |
| HSCN | -599 |
| $TS_{iso}$ | -372 |
| HCN + S | -361 |
| HNC + S | -301 |
| NH + CS | -115 |
| H + NCS | -274 |

### *A5.12 The S + $c-C_3H_2$ reaction*

We have found no barrier for S(3P) addition to $c-C_3H_2$ (the geometry is shown below) at the M06-2X/cc-pVTZ, MP2/cc-pVTZ and CCSD(T)/cc-pVTZ levels. In each case, the geometry of $c-C_3H_2$ was fixed at the isolated $c-C_3H_2$. Then the potential energy curves are not the minimum potential except for S atoms at an infinite distance. The absence of a barrier demonstrates that this reaction should occur. The branching ratios are delicate to estimate as for S(3P) reactions with unsaturated closed shell molecules, intersystem crossing may play a role (as for O + propene and O + allene reactions (Leonori et al. 2011, 2015)) and may lead to $C_2H_2$ + CS formation. We consider 50% of reaction on the triplet surface leading only to $HC_3S$ + H and 50% of intersystem crossing leading ultimately to CS + $C_2H_2$.

### *A5.13 The s-N + s-HCS reaction*

The first step of the N + HCS reaction in the gas phase and on grain is assumed to be N-C bond formation without a barrier as HCS is a radical with the lone electron localized on the carbon atom. There is then the formation of the NC(H)S species which is indeed the Transition State ($TS_{iso}$) for the isomerization between HNCS and HSCN with 372 kJ/mol of excess energy.

In the gas phase the large amount of energy above the bimolecular exit channel will lead to dissociation forming mainly HCN + S and eventually some NH + CS and H + NCS. On grains, we assume that dissipation of the excess energy will be efficient enough to avoid dissociation leading either to HNCS or/and HSCN (even if some HNC + S are likely also produced). We consider that typical time-scales for interconversion is shorter than for relaxation through surface interaction. Thus isomerization of HNCS**/HSCN** leads to equilibrated isomeric abundances at each internal energy. The final balance is determined at or near the effective barrier to isomerization, which corresponds to the energy of the transition state. The ratio between the isomeric forms are then given by the ratio of the rovibrational densities of states of the isomers at the barrier to

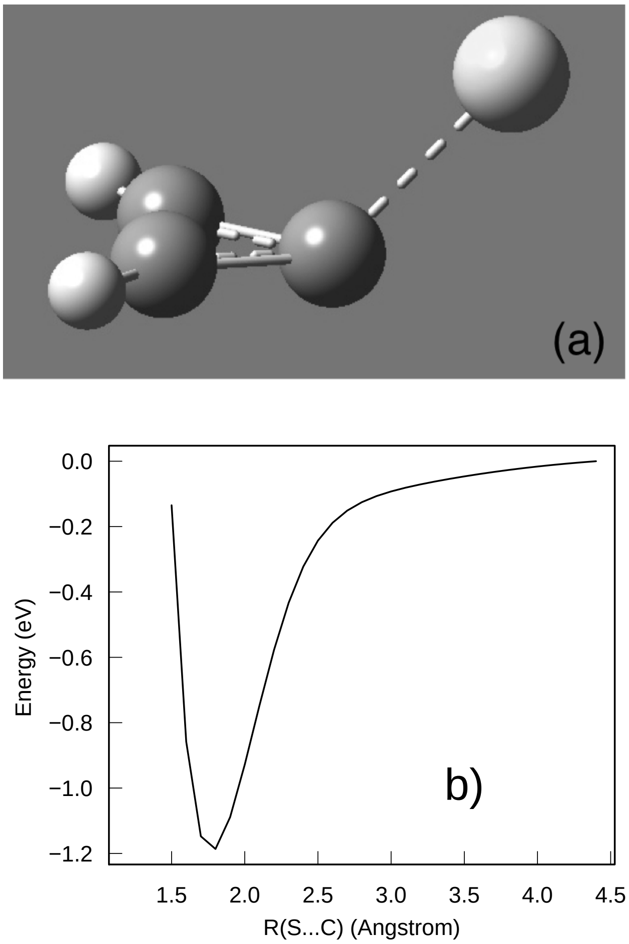


**Figure A12.** (a) Most favorable S attack geometry ; (b) Non relaxed potential energy curve at CCSD(T)/cc-pVTZ for the S + c-$C_3H_2$ reaction.

isomerization calculated using the MESMER program, the isomerization transition state being characterized at the DFT level shown in Figure A14.

| Species (Energy, hartree) | Relative energies (kJ/mol) | Geometries | Frequencies $(cm^{-1})$ |
|---|---|---|---|
| 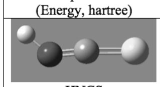 HNCS (-491.615021) | 0 | C 0.495921 0.006919 -0.000008<br>S -1.075582 0.008336 0.000001<br>N 1.683282 -0.102642 0.000003<br>H 2.450808 0.543611 0.000005 | 436, 498, 566, 887, 2094, 3723 |
| 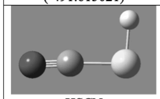 HSCN (-491.600573) | +37.9 | C 0.699105 0.005712 0.000005<br>N 1.848680 0.007482 -0.000002<br>S -0.998201 -0.083468 -0.000001<br>H -1.164171 1.248845 -0.000001 | 349, 407, 713, 984, 2350, 2736 |
| 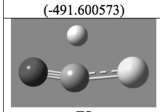 TS (-491.514082) | +265.0 | C 0.000000 0.632489 0.000000<br>S -0.266555 -1.011394 0.000000<br>N 0.446558 1.732325 0.000000<br>H 1.138975 0.261100 0.000000 | 388, 460, 753, 2059, 2449, 1387i |

**Figure A13.** Relative energies at the M06-2X/cc-pVTZ level (in kJ/mol at 0 K including ZPE) with respect to the HNCS energy, geometries and frequencies (in $cm^{-1}$, unscaled) of the various stationary points for the HNCS/HSCN isomerization. The absolute energies at the M06-2X/cc-pVTZ level including ZPE in hartree are also given in column 1.

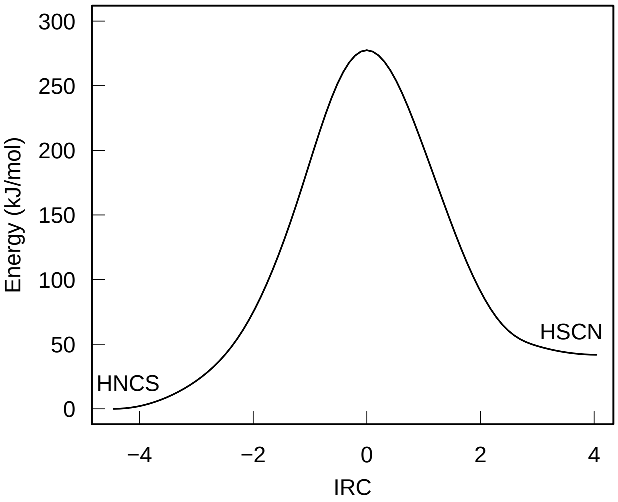


**Figure A14.** Intrinsic Reaction Coordinate (minimum energy path) at M06-2X/cc-pVTZ for the HNCS/HSCN isomerization

## APPENDIX B: SUMMARY OF SULPHUR COMPOUNDS REACTIONS REVIEW

In the following we describe the reactions added or reviewed in our network. The columns of the table contain (for a given reaction):

- the enthalpy of reaction $\Delta E$;

- $\alpha$, $\beta$, and $\gamma$ are the coefficient used to compute the modified Arrhenius reaction rate $k(T) = \alpha(T/300)^{\beta} \times \exp(-\gamma/T)$ (in cm$^3$.molecule$^{-1}$.s$^{-1}$). In some specific cases described below, they are used in another formulation of the reaction rate;

- $F_0$ and $g$ are respectively the uncertainty parameter and the expansion parameter, used to compute the temperature-dependence of the uncertainty factor $F(T)$ (see Sander et al. 2011).

For reactions between ions and neutral species with a dipole moment (indicated by the mention 'Ionpol' in the comments section of the table), the reaction rate coefficients are computed using the Su-Chesnavich capture approach (see discussions in Woon & Herbst 2009; Wakelam et al. 2010). In that case the reaction rate is expressed using two formulas, one for lower and one for higher temperatures. The temperature at which we change formula is computed by the relation:

$$T_m = \frac{\mu_D^2}{(8\alpha_p k_B)} \tag{B1}$$

where $\mu_D$ is the dipole moment (in statC.cm) , $\alpha_p$ the dipole polarizability (in cm$^3$) and $k_B$ the Boltzmann constant (in erg.K$^{-1}$). Hence the reaction rate (in cm$^3$.molecule$^{-1}$.s$^{-1}$) is computed following:

$$k_{T\leq T_m} = \alpha\beta(0.62 + 0.4767\gamma(300/T)^{0.5}) \tag{B2}$$

$$k_{T>T_m} = \alpha\beta(1 + 0.0967\gamma(300/T)^{0.5} + (\gamma^2/10.526)\dot{(}300/T)) \tag{B3}$$

All of these formalisms are described in Wakelam et al. (2012).

**Table B1 :** Table of the sulfur compounds reactions added or reviewed in our network.

| | Reaction | ΔE kJ/mol | α | β | γ | $F_0$ | g | Comments |
|---|---|---|---|---|---|---|---|---|
| 1. | $He^+$ + HNCS → $HNCS^+$ + He<br>→ HNC + $S^+$ + He<br>→ HCN + $S^+$ + He<br>→ H + CN + $S^+$ + He<br>→ $NH^+$ + CS + He | -1430<br>-1052<br>-1087<br>-571<br>-555 | 0.1<br>0.30<br>0.20<br>0.30<br>0.10 | 3.0e-9<br>3.0e-9<br>3.0e-9<br>3.0e-9<br>3.0e-9 | 2.92<br>2.92<br>2.92<br>2.92<br>2.92 | 3<br>3<br>3<br>3<br>3 | 0<br>0<br>0<br>0<br>0 | KIDA, Ionpol1-2 ($T_m$ = 638 K). (Gronowski & Kolos 2014) |
| 2. | $He^+$ + HSCN → $HSCN^+$ + He<br>→ $SH^+$ + CN + He<br>→ H + $NCS^+$ + He | -1329<br>-950<br>-1012 | 0.20<br>0.40<br>0.40 | 2.8e-9<br>2.8e-9<br>2.8e-9 | 5.17<br>5.17<br>5.17 | 3<br>3<br>3 | 0<br>0<br>0 | KIDA, Ionpol1 ($T_m$ = 2005 K). (Gronowski & Kolos 2014) |
| 3. | $He^+$ + HCNS → $HCNS^+$ + He<br>→ HCN + $S^+$ + He<br>→ HNC + $S^+$ + He<br>→ H + CN + $S^+$ + He<br>→ $CH^+$ + NS + He | -1506<br>-1252<br>-1217<br>-718<br>-734 | 0.10<br>0.30<br>0.20<br>0.20<br>0.20 | 2.7e-9<br>2.7e-9<br>2.7e-9<br>2.7e-9<br>2.7e-9 | 5.45<br>5.45<br>5.45<br>5.45<br>5.45 | 3<br>3<br>3<br>3<br>3 | 0<br>0<br>0<br>0<br>0 | Capture rate theory, Ionpol1 ($T_m$ = 2075 K). |
| 4. | $H^+$ + $H_2S$ → $H_2S^+$ + H<br>→ $HS^+$ + $H_2$ | -304<br>-364 | 0.85<br>0.15 | 4.51e-9<br>4.51e-9 | 1.77<br>1.77 | 2<br>2 | 0<br>0 | KIDA, Ionpol1-2 ($T_m$ = 233 K). (Smith *et al.* 1992) |
| 5. | $H^+$ + CS → $CS^+$ + H | -211 | 1.0 | 4.89e-9 | 3.28 | 2 | 0 | KIDA, Ionpol1 ($T_m$ = 800 K). |
| 6. | $H^+$ + $C_2S$ → $C_2S^+$ + H | -298 | 1.0 | 6.2e-9 | 4.12 | 3 | 0 | KIDA, Ionpol1 ($T_m$ = 800 K). |
| 7. | $H^+$ + $C_3S$ → $C_3S^+$ + H | | 1.0 | 7.33e-9 | 4.39 | 3 | 0 | KIDA, Ionpol1 ($T_m$ = 800 K). |
| 8. | $H^+$ + SO → $SO^+$ + H | -288 | 1.0 | 4.38e-9 | 2.93 | 2.0 | 0 | KIDA, Ionpol1 ($T_m$ = 800 K). |
| 9. | $H^+$ + $SO_2$ → $SO_2^+$ + H<br>→ $SO^+$ + OH | -122<br>-196 | 0.5<br>0.5 | 4.2e-9<br>4.2e-9 | 3.1<br>3.1 | 2.0<br>2.0 | 0<br>0 | Capture rate theory, Ionpol1-2 ($T_m$ = 654 K). |
| 10. | $H^+$ + $H_2CS$ → $H_2CS^+$ + H<br>→ $HCS^+$ + $H_2$<br>→ $CS^+$ + H + $H_2$ | -408<br>-633<br>-416 | 0.25<br>0.50<br>0.25 | 5.3e-9<br>5.3e-9<br>5.3e-9 | 2.61<br>2.61<br>2.61 | 2<br>2<br>2 | 0<br>0<br>0 | Capture rate constant with branching ratio deduced from $H^+$ + $H_2CO$ from (Sen *et al.* 1992) considering that $H_2CS^+$ will lead partly to $H_2$ + $CS^+$ |
| 11. | $H^+$ + $CH_3SH$ → $CH_3S^+$ + $H_2$<br>→ $CH_3^+$ + $H_2S$<br>→ $HCS^+$ + $H_2$ + $H_2$ | | 0.50<br>0.25<br>0.25 | 5.5e-9<br>5.5e-9<br>5.5e-9 | 2.3<br>2.3<br>2.3 | 1.4<br>1.4<br>1.4 | 0<br>0<br>0 | Capture rate theory, branching ratio from (Anicich 2003). |
| 12. | $H^+$ + HNCS → $HNCS^+$ + H<br>→ HNC + $SH^+$<br>→ NH + $HCS^+$<br>→ $H_2$ + $NCS^+$ | -355<br>-319<br>-259<br>-208 | 0.40<br>0.30<br>0.20<br>0.10 | 5.9e-9<br>5.9e-9<br>5.9e-9<br>5.9e-9 | 2.92<br>2.92<br>2.92<br>2.92 | 3<br>3<br>3<br>3 | 0<br>0<br>0<br>0 | (Gronowski & Kolos 2014), Ionpol1-2 ($T_m$ = 638 K). |

| | | | | | | | | |
|---|---|---|---|---|---|---|---|---|
| 13. | $H^+$ + HSCN → $HSCN^+$ + H<br>→ HCN + $SH^+$<br>→ HNC + $SH^+$<br>→ $H_2$ + $NCS^+$ | -254<br>-410<br>-355<br>-363 | 0.40<br>0.30<br>0.20<br>0.10 | 5.46e-9<br>5.46e-9<br>5.46e-9<br>5.46e-9 | 5.17<br>5.17<br>5.17<br>5.17 | 3<br>3<br>3<br>3 | 0<br>0<br>0<br>0 | Capture rate theory, Ionpol1 ($T_m$ = 2005 K). |
| 14. | $H^+$ + HCNS → $HCNS^+$ + H<br>→ $CH_2^+$ + NS<br>→ $SH^+$ + HCN | -322<br>-117<br>-410 | 0.20<br>0.30<br>0.50 | 5.3e9<br>5.3e-9<br>5.3e-9 | 5.45<br>5.45<br>5.45 | 3<br>3<br>3 | 0<br>0<br>0 | Capture rate theory, Ionpol1 ($T_m$ = 2075 K). |
| 15. | $H^+$ + $NH_2CHS$ → $NH_3$ + $HCS^+$<br>→ $NH_2CHS^+$ + H | | 5.0e-9<br>0 | 0 | 0 | 3 | 0 | Similar rate constant than $H^+$ reactions (Anicich 2003) considering no barrier for this reaction |
| 16. | $H^+$ + $NH_2CH_2SH$→ $NH_3$ + $H_3CS^+$<br>→ $NH_2CH_2SH^+$ + H | | 5.0e-9<br>0 | 0 | 0 | 3 | 0 | Similar rate constant than $H^+$ reactions (Anicich 2003) considering no barrier for this reaction |
| 17. | H + SH → $H_2$ + S | -79 | 2.5e-11 | 0 | 0 | 5 | 0 | (Cupitt & Glass 1975, Peng *et al.* 1999, Maiti *et al.* 2004, Nicholas *et al.* 1979, Tiee *et al.* 1981, Bradley *et al.* 1973). |
| 18. | H + $H_2S$ → $H_2$ + HS | -56 | 1.50e-11 | 0 | 860 | 1.6 | 200 | Rate constant valid in the 190-464 K range (Kurylo *et al.* 1971). (Peng et al. 1999) proposed a slightly different expression valid only in the 298-598 K range (with similar rate constant value in that range). |
| 19. | H + $HS^+$ → $H_2$ + $S^+$ | -85 | 1.1e-10 | 0 | 0 | 1.6 | 0 | (Millar *et al.* 1986) |
| 20. | H + $H_2S^+$ → $H_2$ + $HS^+$ | -60 | 2.2e-10 | 0 | 0 | 1.6 | 0 | (Millar et al. 1986) |
| 21. | H + $H_3S^+$ → $H_2$ + $H_2S^+$ | -33 | 6.0e-11 | 0 | 0 | 1.6 | 0 | (Millar et al. 1986) |
| 22. | H + $H_2C_2S^+$ → $HC_2S^+$ + $H_2$ | -35 | 1.0e-10 | 0 | 0 | 3 | 0 | Capture rate theory |
| 23. | H + $C_2S$ → CH + CS<br>→ S + $C_2H$ | +47<br>+20 | “0”<br>“0” | | | | | No exothermic bimolecular exit channel leading to negligible rate constant at low temperature. |
| 24. | H + HCS → $H_2$ + CS<br>→ $H_2CS$ | -215<br>-381 | 1.5e-10<br>0 | 0 | 0 | 2 | 0 | Capture rate theory |
| 25. | H + $CH_3S$ → $H_2$ + $H_2CS$<br>→ $CH_3$ + SH | -210<br>-49 | 3.0e-11<br>3.0e-12 | 0<br>0 | 0<br>0 | 1.6<br>1.6 | 100<br>100 | Capture rate theory |
| 26. | H + $CH_2SH$ → $H_2$ + $H_2CS$<br>→ $CH_3$ + SH | -246<br>-85 | 1.0e-11<br>1.6e-10 | 0<br>0 | 0<br>0 | 3<br>2 | 0<br>0 | Capture rate theory |
| 27. | H + $HC_3S$ → $H_2$ + $C_3S$<br>→ $C_2H_2$ + CS | -121<br>-177 | 1.0e-11<br>3.0e-11 | 0<br>0 | 0<br>0 | 5<br>5 | 0<br>0 | Capture rate theory. |
| 28. | H + $HSO^+$ → $SO^+$ + $H_2$<br>→ O + $H_2S^+$<br>→ $HS^+$ + OH | -173<br>+66<br>+13 | 2.0e-10<br>0<br>0 | 0 | 0 | 2 | 0 | By comparison with H + $H_2S^+$ |

| | | | | | | | | |
|---|---|---|---|---|---|---|---|---|
| | → $S + H_2O^+$<br>→ $S^+ + H_2O$ | +81<br>-136 | 0<br>0 | | | | | |
| 29. | $H_2 + S^+$ → $H + HS^+$<br>→ $H_2S^+ + h\nu$ | +85 | 8.0e-11<br>1.0e-17 | 0<br>-0.2 | 9860<br>0 | 1.8<br>10 | 1000<br>0 | (Millar et al. 1986), experimental determination. The $H_2S^+ + h\nu$ rate constant is from KIDA. |
| 30. | $H_2 + HS^+$ → $H + H_2S^+$<br>→ $H_3S^+ + h\nu$ | +60 | 7.0e-11<br>1.4e-16 | 0<br>-0.6 | 6380<br>0 | 1.8<br>10 | 600<br>0 | (Millar et al. 1986), experimental determination. The $H_3S^+ + h\nu$ rate constant is from KIDA. |
| 31. | $H_2 + H_2S^+$ → $H + H_3S^+$ | +33 | 5.0e-12 | 0 | 2900 | 2 | 300 | (Millar et al. 1986), experimental determination |
| 32. | $H_2 + CS^+$ → $H + HCS^+$ | -141 | 4.3e-10 | 0 | 0 | 1.4 | 0 | (Anicich 2003) |
| 33. | $H_2 + C_2S^+$ → $H + HC_2S^+$ | -127 | 4.3e-10 | 0 | 0 | 2 | 0 | Same as $CS^+ + H_2$ |
| 34. | $H_2 + C_3S^+$ → $H + HC_3S^+$ | -150 | 4.3e-10 | 0 | 0 | 2 | 0 | Same as $CS^+ + H_2$ |
| 35. | $C^+ + S$ → $S^+ + C$ | -68 | 1.3e-9 | 0 | 0 | 10 | 0 | See KIDA datasheet. Large uncertainty. |
| 36. | $C^+ + H_2S$ → $H_2S^+ + C$<br>→ $HCS^+ + H$ | -77<br>-541 | 0.252<br>0.748 | 1.49e-9<br>1.49e-9 | 1.77<br>1.77 | 2<br>2 | 0<br>0 | KIDA, Ionpol1-2 ($T_m$ = 253 K). See also (Anicich 2003). |
| 37. | $C^+ + SO$ → $CO + S^+$<br>→ $CO^+ + S$<br>→ $CS^+ + O$<br>→ $C + SO^+$ | -642<br>-290<br>-186<br>-93 | 0.25<br>0.25<br>0.25<br>0.25 | 1.4e-9<br>1.4e-9<br>1.4e-9<br>1.4e-9 | 2.93<br>2.93<br>2.93<br>2.93 | 3<br>3<br>3<br>3 | 0<br>0<br>0<br>0 | KIDA, Ionpol1-2 ($T_m$ = 643 K). |
| 38. | $C^+ + SO_2$ → $SO^+ + CO$ | -619 | 1 | 1.44e-9 | 2.96 | 2 | 0 | KIDA, Ionpol1-2 ($T_m$ = 654 K). See also (Anicich 2003) |
| 39. | $C^+ + CH_3SH$ → $CH_3^+ + HCS$<br>→ $CH_3S^+ + CH$ | -397 | 0.80<br>0.20 | 1.75e-9<br>1.75e-9 | 2.33<br>2.33 | 3<br>3 | 0<br>0 | Capture rate theory, Ionpol1-2 ($T_m$ = 407 K). Branching ratio deduced from $C^+ + CH_3OH$ reaction (Anicich 2003). |
| 40. | $C^+ + HNCS$ → $HNCS^+ + C$<br>→ $HNC^+ + CS$<br>→ $CH^+ + NCS$ | -139<br>-285<br>-15 | 0.20<br>0.80<br>0 | 1.85e-9<br>1.85e-9 | 2.92<br>2.92 | 3<br>3 | 0<br>0 | (Gronowski & Kolos 2014), Ionpol1-2 ($T_m$ = 638 K). |
| 41. | $C^+ + HSCN$ → $HSCN^+ + C$<br>→ $HCS^+ + CN$ | -38<br>-479 | 0.20<br>0.80 | 1.71e-9<br>1.71e-9 | 5.17<br>5.17 | 3<br>3 | 0<br>0 | (Gronowski & Kolos 2014), Ionpol1 ($T_m$ = 2005 K). |
| 42. | $C^+ + HCNS$ → $HCNS^+ + C$<br>→ $HCN^+ + CS$<br>→ $HCN + CS^+$ | -219<br>-344<br>-552 | 0.20<br>0.20<br>0.60 | 1.6e-9<br>1.6e-9<br>1.6e-9 | 5.45<br>5.45<br>5.45 | 3<br>3<br>3 | 0<br>0<br>0 | Capture rate theory, Ionpol1 ($T_m$ = 2075 K). |
| 43. | $C^+ + NH_2CHS$ → $H + HCN + HCS^+$ | | 1.0 | 2.0e-9 | 5.6 | 3 | 0 | Capture rate theory, Ionpol1 ($T_m$ = 2000 K). |
| 44. | $C^+ + NH_2CH_2SH$ → $CH_2NH_2 + HCS^+$ | | 1.0 | 2.0e-9 | 1.3 | 3 | 0 | Capture rate theory, Ionpol1-2 ($T_m$ = 142 K). |
| 45. | $C^+ + C_2S$ → $C_2S^+ + C$<br>→ $C_3 + S^+$ | -78<br>-304<br>-53 | 0.2<br>0.7<br>0 | 1.95e-9<br>1.95e-9 | 4.12<br>4.12 | 3<br>3 | 0<br>0 | KIDA, Ionpol1 ($T_m$ = 800 K). There are no data for this reaction but by comparison with other $C^+$ reaction, the charge exchange is likely a minor but |

| | | | | | | | | |
|---|---|---|---|---|---|---|---|---|
| | → $C_3^+$ + S<br>→ CS + $C_2^+$ | -155 | 0.1 | 1.95e-9 | 4.12 | 3 | 0 | non negligible channel. |
| 46. | $C^+$ + $C_3S$ → $C_3S^+$ + C<br>→ $C_4^+$ + S<br>→ $C_3^+$ + CS<br>→ $C_3$ + $CS^+$<br>→ $C_2^+$ + $C_2S$ | -115<br>-38<br>-156<br>-183<br>+324 | 0.25<br>0.25<br>0.25<br>0.25<br>0 | 2.28e-9<br>2.28e-9<br>2.28e-9<br>2.28e-9 | 4.39<br>4.39<br>4.39<br>4.39 | 2<br>2<br>2<br>2 | 0<br>0<br>0<br>0 | KIDA, Capture rate theory, Ionpol1 ($T_m$ = 800 K). Enthalpy of reaction calculated at M06-2X/aug-cc-pVTZ level (this work), except for $C_4^+$ (Gingerich *et al.* 1994, Belau *et al.* 2007, Hochlaf *et al.* 2007), $CS^+$ (NIST) and $C_3^+$ (Nicolas *et al.* 2005) |
| 47. | C + $HS^+$ → H + $CS^+$<br>→ S + $CH^+$<br>→ CH + $S^+$<br>→ HS + $C^+$ | -272<br>+38<br>+11<br>+80 | 9.9e-10 | 0 | 0 | 2 | 0 | KIDA |
| 48. | C + HS → H + CS | -345 | 2.0e-10 | 0 | 0 | 2 | 0 | Capture rate theory |
| 49. | C + $H_2S^+$ → H + $HCS^+$ | 453 | 1.0e-9 | 0 | 0 | 2 | 0 | KIDA |
| 50. | C + $H_2S$ → HCS + H | -187 | 2.5e-10 | 0 | 0 | 1.4 | 7 | (Deeyamulla & Husain 2006, Galland *et al.* 2001) |
| 51. | C + SO → CO + S<br>→ CS + O | -562<br>-188 | 1.0e-10<br>1.0e-10 | 0<br>0 | 0<br>0 | 2<br>2 | 21<br>21 | Capture rate theory |
| 52. | C + NS → CN + S | -290 | 2.0e-10 | 0 | 0 | 1.6 | 0 | Capture rate theory |
| 53. | C + $NS^+$ → CN + $S^+$<br>→ N + $CS^+$ | -137<br>-3 | 6.0e-10<br>0 | 0 | 0 | 3 | 0 | Capture rate theory |
| 54. | C + $SO^+$ → CO + $S^+$<br>→ CS + $O^+$<br>→ $C^+$ + SO | -549<br>+128<br>+93 | 6.0e-10<br>0<br>0 | 0 | 0 | 2 | 0 | Capture rate theory |
| 55. | C + HCO → $C_2O$ + H<br>→ CO + CH | -159<br>-275 | 2.0e-11<br>1.8e-10 | 0<br>0 | 0<br>0 | 3<br>0 | 0<br>0 | Capture rate theory |
| 56. | C + HCS → H + $C_2S$<br>→ S + $C_2H$<br>→ CS + CH | -224<br>-172<br>-118 | 2.0e-10<br>1.0e-10<br>0 | 0<br>0 | 0<br>0 | 3<br>3 | 0<br>0 | Capture rate theory |
| 57. | C + $H_2CS$ → $CH_2$ + CS<br>→ H + HCCS | -169<br>-265 | 1.0e-10<br>2.0e-10 | 0<br>0 | 0<br>0 | 3<br>3 | 0<br>0 | Capture rate theory, similar to C + $H_2CO$ (Husain & Ioannou 1999). |
| 58. | C + $CH_3S$ → $CH_3$ + CS | -394 | 3.0e-10 | 0 | 0 | 2 | 0 | Capture rate theory |
| 59. | C + $CH_2SH$ → $CH_3$ + CS | -430 | 3.0e-10 | 0 | 0 | 2 | 0 | Capture rate theory |
| 60. | C + $CH_3SH$ → $CH_3$ + HCS | -250 | 3.0e-10 | 0 | 0 | 0 | 0 | Capture rate theory, similar to C + $CH_3OH$ (Shannon *et al.* 2014). |
| 61. | C + $SO_2$ → CO + SO | -568 | 8.0e-11 | 0 | 0 | 2 | 0 | (Dorthe *et al.* 1991, Deeyamulla & Husain 2006). |
| 62. | C + OCS → CS + CO | -387 | 1.0e-10 | 0 | 0 | 2 | 21 | (Dorthe et al. 1991, Deeyamulla & Husain 2006). |

| | | | | | | | | |
|---|---|---|---|---|---|---|---|---|
| 63. | C + HNCS → HNC + CS<br>→ HCN + CS | -356<br>-409 | 1.0e-10<br>1.0e-10 | 0<br>0 | 0<br>0 | 2<br>2 | 0<br>0 | Capture rate theory |
| 64. | C + HSCN → HCN + CS | -447 | 2.0e-10 | 0 | 0 | 2 | 0 | Capture rate theory |
| 65. | C + HCNS → HCN + CS | -556 | 2.0e-10 | 0 | 0 | 2 | 0 | Capture rate theory |
| 66. | C + $C_2O$ → $C_2$ + CO<br>→ $C_3$ + O | -374<br>-31 | 2.0e-10<br>0 | 0 | 0 | 3 | 10 | Capture rate theory, assuming no barrier for the singlet and the triplet surfaces |
| 67. | C + $C_2S$ → $C_2$ + CS | -208 | 2.0e-10 | 0 | 0 | 3 | 0 | Capture rate theory, assuming no barrier for the singlet and the triplet surfaces |
| 68. | C + HCCS → H + $C_3S$<br>→ $C_2H$ + CS | -276<br>-217 | 1.0e-10<br>1.0e-10 | 0<br>0 | 0<br>0 | 3<br>3 | 0<br>0 | Capture rate theory |
| 69. | C + $H_2CCS$ → $C_2H_2$ + CS | -385 | 3.0e-10 | 0 | 0 | 3 | 0 | Capture rate theory |
| 70. | C + $NH_2CHS$ → $CH_2NH$ + CS | -381 | 3.0e-10 | 0 | 0 | 3 | 0 | Capture rate theory |
| 71. | C + $NH_2CHO$ → $CH_2NH$ + CO | -537 | 3.0e-10 | 0 | 0 | 3 | 0 | Capture rate theory |
| 72. | C + $NH_2CH_2SH$ → $CH_3NH_2$ + CS | -441 | 3.0e-10 | 0 | 0 | 3 | 0 | Capture rate theory |
| 73. | C + $C_3S$ → $C_3$ + CS | -176 | 3.0e-10 | 0 | 0 | 3 | 0 | Capture rate theory |
| 74. | C + $HC_3S$ → $C_2H$ + $C_2S$<br>→ H + $C_4S$<br>→ l-$C_3H$ + CS<br>→ c-$C_3H$ + CS | -71<br>-206<br>-186 | 0<br>5.0e-11<br>5.0e-11<br>5.0e-11 | 0<br>0<br>0<br>0 | 0<br>0<br>0<br>0 | 0<br>5<br>3<br>3 | 0<br>0<br>0<br>0 | Capture rate theory |
| 75. | C + $C_4S$ → $C_4$ + CS | -151 | 2.0e-10 | 0 | 0 | 3 | 0 | Capture rate theory |
| 76. | CH + CS → $C_2S$ + H<br>→ $C_2H$ + S | -106<br>-54 | 1.5e-10<br>5.0e-11 | 0<br>0 | 0<br>0 | 3<br>3 | 0<br>0 | By comparison with CH + CO (Le Picard *et al.* 1998) |
| 77. | CH + $C_3S$ → H + $C_4S$<br>→ CS + l-$C_3H$ | -182<br>-163 | 1.0e-10<br>1.0e-10 | 0<br>0 | 0<br>0 | 3<br>3 | 0<br>0 | By comparison with CH + alkenes, alkynes |
| 78. | $CH_2$ + NS → HCNS + H | -193 | 4.0e-11 | 0 | 0 | 3 | 0 | By comparison with $CH_2$ + NO (Fikri *et al.* 2001, Eshchenko *et al.* 2002) |
| 79. | $CH_3^+$ + CS → $CH_3CS^+$ + hν | -485 | 1.0e-13 | -1.0 | 0 | 3 | 0 | By comparison with $CH_3^+$ + CO |
| 80. | $CH_3^+$ + $H_2S$ → $CH_3S^+$($CH_2SH^+$) + $H_2$ | -178 | 1.00 | 2.48e-10 | 1.77 | 1.6 | 0 | Ionpol1-2 ($T_m$ = 253 K).. See also (Anicich 2003). KIDA consider one $CH_3S^+$/$CH_2SH^+$ isomer which is indeed $CH_2SH^+$ (the more stable form) named $CH_3S^+$! |
| 81. | $C_2H$ + CS → $C_3S$ + H | -62 | 2.0e-10 | 0 | 0 | 3 | 0 | By comparison with $C_2H$ + CO (Lander *et al.* 1990, Petrie 1996) |
| 82. | $C_2H$ + $C_3S$ → H + $C_5S$ | -98 | 1.0e-10 | 0 | 0 | 3 | 0 | By comparison with CH + alkenes, alkynes. |

| | | | | | | | | |
|---|---|---|---|---|---|---|---|---|
| | | → $CS + C_4H$ | -58 | 1.0e-10 | 0 | 0 | 3 | 0 |
| 83. | $C_2H + CH_3SH$ | → $C_2H_2 + CH_3S$<br>→ $C_2H_2 + CH_2SH$ | -186<br>-150 | 1.0e-10<br>3.0e-11 | 0<br>0 | 0<br>0 | 3<br>3 | 0<br>0 | By comparison with CN + $CH_3SH$ and $C_2H$ + $CH_3OH$ |
| 84. | $C_2H_3 + CS$ | → $H + H_2C_3S$ | -33 | 3.0e-12 | 0 | 300 | 3 | 300 | See appendix A. |
| 85. | $CN + CH_3SH$ | → $HCN + CH_3S$<br>→ $HCN + CH_2SH$ | -178<br>-142 | 2.0e-10<br>7.0e-11 | 0<br>0 | 0<br>0 | 1.6<br>1.6 | 0<br>0 | (Decker & Macdonald 2001) |
| 86. | $N + HS^+$ | → $H + NS^+$<br>→ $S + NH^+$<br>→ $S^+ + NH$ | -269<br>+313<br>+15 | 7.4e-10<br>0<br>0 | 0 | 0 | 2 | 0 | KIDA |
| 87. | $N + HS$ | → $H + NS$ | -97 | 1.0e-10 | 0 | 0 | 2 | 0 | KIDA |
| 88. | $N + H_2S^+$ | → $H_2 + NS^+$<br>→ $NH + HS^+$<br>→ $NH^+ + HS$ | -329<br>+40<br>+332 | 7.90e-10<br>0<br>0 | 0 | 0 | 2 | 0 | KIDA |
| 89. | $N + NS$ | → $N_2 + S$ | -485 | 4.0e-11 | -0.2 | 20 | 3 | 0 | Equal to N + NO rate constant |
| 90. | $N + NS^+$ | → $N_2 + S^+$ | -328 | 6.0e-10 | 0 | 0 | 3 | 0 | Capture rate theory |
| 91. | $N + SO^+$ | → $NO^+ + S$<br>→ $NO + S^+$<br>→ $O + NS^+$ | -210<br>-104<br>-90 | 0<br>0<br>5.0e-11 | <br><br>0 | <br><br>0 | <br><br>3 | <br><br>0 | Indirect measurement from (Fehsenfeld & Ferguson 1973). It should be noted that considering the exothermicity is a strange result. |
| 92. | $N + HCS$ | → $HCN + S$ | -361 | 1.0e-10 | 0.17 | 0 | 2 | 0 | Capture rate theory, see also appendix A. |
| 93. | $N + CH_3S$ | → $CH_3 + NS$ | -144 | 6.00e-11 | 0 | 0 | 2 | 0 | Capture rate theory |
| 94. | $N + CH_2SH$ | → $HCN + H_2S$ | -509 | 6.00e-11 | 0 | 0 | 2 | 0 | Capture rate theory |
| 95. | N + HCCS | → HCN + CS | -65 | 8.0e-11 | 0 | 0 | 3 | 0 | Capture rate theory |
| 96. | $N + C_2S$ | → CN + CS | -367 | 3.0-11 | 0.17 | 0 | 3 | 0 | Capture rate theory |
| 97. | $N + HC_3S$ | → $HCN + C_2S$ | -252 | 1.0e-10 | 0 | 0 | 3 | 0 | Capture rate theory |
| 98. | $N + C_4S$ | → $CN + C_3S$<br>→ $C_3N + CS$ | -235<br>-269 | 1.5e-11<br>1.5e-11 | 0.17<br>0.17 | 0<br>0 | 3<br>3 | 0<br>0 | Capture rate theory |
| 99. | NH + CS | → HNC + S | -187 | 1.0e-11 | 0 | 1200 | 3 | 0 | See appendix A. |
| 100. | NH + HCS | → HNCS + H | -311 | 5.0e-11 | 0 | 0 | 3 | 0 | Capture rate theory |
| 101. | $NH + HCS^+$ | → $HNCS^+ + H$ | -96 | 1.0 | 7.2e-10 | 5.1 | | | Capture rate theory, Ionpol1 ($T_m$ = 1729 K). |
| 102. | NH + CCS | → HCN + CS<br>→ HNC + CS | -549<br>-494 | 2.0e-11<br>2.0e-11 | 0<br>0 | 0<br>0 | 3<br>3 | 0<br>0 | Capture rate theory |
| 103. | $NH_2^+ + CS$ | → $H_2NCS^+ + h\nu$ | -658 | 2.4e-11 | -1.0 | 0 | 10 | 0 | By comparison with $NH_2^+$ + CO (Adams *et al.* 1980). Very minor reaction in dense molecular clouds. |
| 104. | $NH_2 + CS$ | → HNCS + H | -147 | 1.0e-12 | 0 | 600 | 3 | 600 | See appendix A. |

| | | | | | | | | |
|---|---|---|---|---|---|---|---|---|
| 105. | $NH_2 + HCS^+$ → $H_2NCS^+ + H$<br>→ $HNCSH^+ + H$ | -118<br>-81 | 0.998<br>0.002 | 9.0e-10<br>9.0e-10 | 4.7<br>4.7 | | | KIDA, Ionpol1 ($T_m$ = 1648 K). (Gronowski & Kolos 2014). |
| 106. | $NH_3^+ + CS$ → $H_2NCS^+ + H$ | -134 | 1.0e-9 | -0.4 | 0 | 3 | 10 | Capture rate theory assuming no barrier in the entrance valley (system isoelectronic to $NH_2 + HCS^+$) |
| 107. | $NH_3 + HCS^+$ → $CS + NH_4^+$ | -57 | 1.0 | 9.5e-10 | 3.8 | | | KIDA, Ionpol1 ($T_m$ = 1068 K). (Gronowski & Kolos 2014) |
| 108. | $O + HS^+$ → $OH + S^+$<br>→ $H + SO^+$ | -80<br>-179 | 2.9e-10<br>2.9e-10 | 0<br>0 | 0<br>0 | 2<br>2 | 0<br>0 | KIDA |
| 109. | $O + HS$ → $H + SO$ | -157 | 1.60e-10 | 0.17 | 0 | 2 | 0 | KIDA (Cupitt & Glass 1975). |
| 110. | $O + H_2S^+$ → $OH + HS^+$<br>→ $H_2 + SO^+$ | -55<br>-239 | 3.1e-10<br>3.1e-10 | 0<br>0 | 0<br>0 | 2<br>2 | 0<br>0 | KIDA |
| 111. | $O + NS$ → $NO + S$<br>→ $SO + N$ | -146<br>-35 | 3.0e-11<br>0.0 | 0 | 0 | 2 | 0 | Equal to high pressure rate constant from the O + NO → $NO_2$ reaction (similar entrance channel) |
| 112. | $O + NS^+$ → $NO^+ + S$<br>→ $NO + S^+$ | -120<br>-14 | 6.1e-10<br>0 | 0 | 0 | 2 | 0 | KIDA |
| 113. | $O + CH_3^+$ → $H_2 + HCO^+$<br>→ $H_2 + HOC^+$<br>→ $H_2CO^+ + H$ | -515<br>-380<br>-193 | 2.05e-10<br>2.05e-10<br>1.0e-15 | 0<br>0<br>0 | 0<br>0<br>0 | 2<br>2<br>10 | 0<br>0<br>0 | (Anicich 2003, Scott *et al.* 2000), the $HCO^+/HOC^+$ ratio is purely arbitrary. The $H_2CO^+ + H$ branching ratio is in fact unknown. |
| 114. | $O + CS$ → $CO + S$ | -377 | 2.61e-10 | 0 | 758 | 1.4 | 300 | (Lilenfeld & Richardson 1977) |
| 115. | $O + CS^+$ → $CO + S^+$<br>→ $CO^+ + S$ | -456<br>-107 | 0<br>6.0e-11 | 0 | 0 | 2 | 0 | KIDA. The reason why $CO + S^+$ branching ratio in KIDA is equal to zero is unknown. However, as $CS^+$ reacts with $H_2$, this reaction is not important in dense molecular clouds. |
| 116. | $O + HCS$ → $H + OCS$<br>→ $HS + CO$<br>→ $OH + CS$<br>→ $S + HCO$ | -471<br>-512<br>-208<br>-224 | 1.0e-10<br>0<br>0<br>0 | 0<br>0 | 0<br>0 | 2<br>2 | 0<br>0 | We favor H + OCS production as the first step is very likely OC(H)S formation which will evolve quickly toward H + OCS in the gas phase using (Rice *et al.* 1993, Rice & Chabalowski 1994). |
| 117. | $O + CH_3S$ → $CH_3 + SO$ | -206 | 4.0e-11 | 0 | 0 | 2 | 0 | Equal to $O + CH_3O$ (Ewig *et al.* 1987) |
| 118. | $O + CH_2SH$ → $H_2CO + HS$<br>→ $H_2CS + OH$ | -370<br>-239 | 4.0e-11<br>4.0e-11 | 0<br>0 | 0<br>0 | 2<br>2 | 0<br>0 | Equal to $O + CH_2OH$ (Grotheer *et al.* 1989) |
| 119. | $O + C_2H_3^+$ → $H_2 + HC_2O^+$<br>→ $H + H_2C_2O^+$<br>→ $CH_3^+ + CO$ | -258<br>-287<br>-394 | 0<br>8.5e-11<br>5.0e-12 | 0<br>0<br>0 | 0<br>0<br>0 | 0<br>2<br>2 | 0<br>0<br>0 | (Scott et al. 2000) |
| 120. | $O + HCNS$ → $HCO + NS$<br>→ $HCN + SO$ | -176<br>-367 | 5.0e-10<br>5.0e-10 | 0<br>0 | 0<br>0 | 4<br>4 | 0<br>0 | See appendix A |

| | | | | | | | | | |
|---|---|---|---|---|---|---|---|---|---|
| 121. | O + HCCS | → HCO + CS | -269 | 1.6e-10 | 0 | 0 | 2 | 0 | Capture rate theory |
| 122. | O + $C_2S$ | → CS + CO | -689 | 9.0e-11 | 0 | 0 | 3 | 0 | Capture rate theory , similar to O + $C_2O$ reaction (Shackleford *et al.* 1972, Bauer *et al.* 1985) |
| 123. | O + $C_3S$ | → CO + $C_2S$ | -370 | 1.94e-11 | 0 | 231 | 3 | 231 | KIDA. See appendix A. |
| 124. | O + $HC_3S$ | → OH + $C_3S$<br>→ HCO + $C_2S$ | -113<br>-122 | 5.0e-11<br>5.0e-11 | 0<br>0 | 0<br>0 | 3<br>3 | 0<br>0 | Capture rate theory |
| 125. | O + $C_4S$ | → $C_3S$ + CO<br>→ CS + $C_3O$ | -557<br>-405 | 9.0e-11<br>1.0e-11 | 0<br>0 | 0<br>0 | 3<br>3 | 0<br>0 | Capture rate theory |
| 126. | OH + CS | → OCS + H<br>→ SH + CO | -237<br>-289 | 1.7e-10<br>3.0e-11 | 0<br>0 | 0<br>0 | 3<br>3 | 0<br>0 | (Adriaens *et al.* 2010, Rice et al. 1993) |
| 127. | OH + SO | → $SO_2$ + H | -66 | 8.2e-11 | 0 | 0 | 1.4 | 3 | (Blitz *et al.* 2000, Jourdain *et al.* 1979) |
| 128. | OH + $H_2S$ | → $H_2O$ + HS | -117 | 4.0e-12 | -0.2 | 0 | 1.4 | 10 | (Lin *et al.* 1985, Mousavipour *et al.* 2003, Ellingson & Truhlar 2007) |
| 129. | OH + $CH_3SH$ | → $H_2O$ + $CH_3S$<br>→ $H_2O$ + $CH_2SH$ | -127<br>-91 | 8.0e-12<br>2.5e-11 | -0.4<br>-0.4 | 0<br>0 | 1.6<br>1.6 | 10<br>10 | (Hynes & Wine 1987, Butkovskaya & Setser 1999). |
| 130. | OH + $C_3S$ | → CO + HCCS<br>→ H + $SC_3O$ | -374<br>-273 | 2.0e-10<br>0 | 0 | 0 | 3 | 0 | Capture rate theory |
| 131. | $S^+$ + CH | → H + $CS^+$ | | 1.0 | 1.12e-9 | 3.33 | 3 | 0 | KIDA, Ionpol1 ($T_m$ = 800 K). |
| 132. | $S^+$ + $CH_2$ | → H + $HCS^+$ | | 1.0 | 1.09e-9 | 1.41 | 3 | 0 | KIDA, Ionpol1-2 ($T_m$ = 149 K). |
| 133. | $S^+$ + $CH_3$ | → H + $H_2CS^+$ | | 3.0e-10 | 0 | 0 | 3 | 0 | Similar to $S^+$ + $CH_4$. |
| 134. | $S^+$ + $CH_4$ | → H + $H_3CS^+$<br>→ $HCS^+$ + $H_2$ + H | | 3.0e-10<br>2.0e-11 | 0<br>0 | 0<br>0 | 1.4<br>1.4 | 0<br>0 | (Anicich 2003) |
| 135. | $S^+$ + $C_2$ | → C + $CS^+$ | | 8.1e-10 | 0 | 0 | 2 | 0 | KIDA |
| 136. | $S^+$ + $C_2H$ | → H + $C_2S^+$ | | 1.0 | 1.34e-9 | 1.34 | 2 | 0 | KIDA, Ionpol1-2 ($T_m$ = 133 K). |
| 137. | $S^+$ + $C_2H_2$ | → H + $HC_2S^+$ | -66 | 9.7e-10 | 0 | 0 | 1.2 | 0 | (Anicich 2003) |
| 138. | $S^+$ + $C_2H_4$ | → $HCS^+$ + $CH_3$<br>→ $CH_3CS^+$ + H | -150<br>-217 | 7.0e-10<br>3.0e-10 | 0<br>0 | 0<br>0 | 1.6<br>1.6 | 0<br>0 | (Anicich 2003) |
| 139. | $S^+$ + c-$C_3H_2$ | → H + $HC_3S^+$ | | 1.0 | 1.2e-9 | 5.54 | 3 | 0 | Capture rate theory, Ionpol1 ($T_m$ = 800 K). |
| 140. | $S^+$ + l-$C_3H_2$ | → H + $HC_3S^+$ | | 1.0 | 1.33e-9 | 6.11 | 3 | 0 | Capture rate theory, Ionpol1 ($T_m$ = 800 K). |
| 141. | $S^+$ + $C_4H$ | → H + $C_4S^+$<br>→ $C_3H^+$ + CS | -147<br>-151 | 0.5<br>0.5 | 1.42e-9<br>1.42e-9 | 1.13<br>1.13 | 4<br>4 | 0<br>0 | KIDA, Ionpol1-2 ($T_m$ = 94 K). |
| 142. | $S^+$ + $C_4H_2$ | → c-$C_3H_2^+$ + CS<br>→ l-$C_3H_2^+$ + CS<br>→ $C_4H^+$ + HS<br>→ H + $HC_4S^+$ | -82<br>+105<br>+247<br>-44 | 1.2e-10<br>0<br>0<br>4.8e-10 | 0<br>0<br>0<br>0 | 0<br>0<br>0<br>0 | 2<br>2<br>2<br>2 | 0<br>0<br>0<br>0 | KIDA |

| | | | | | | | | |
|---|---|---|---|---|---|---|---|---|
| | → $S + C_4H_2^+$ | -18 | 7.2e-10 | 0 | 0 | 2 | 0 | |
| 143. | $S^+ + NH_3$ → $S + NH_3^+$ | | 1.0 | 6.4e-10 | 3.65 | 1.4 | 0 | Capture rate theory, Ionpol1 ($T_m$ = 800 K). See also (Anicich 2003) |
| 144. | $S^+ + O_2$ → $SO^+ + O$ | | 1.8e-11 | 0 | 0 | 1.4 | 7 | (Anicich 2003) |
| 145. | $S^+ + NO$ → $S + NO^+$ | | 1.0 | 4.0e-10 | 0.411 | 1.4 | 7 | Capture rate theory, Ionpol1-2 ($T_m$ = 12 K). See also (Anicich 2003) |
| 146. | $S^+ + H_2S$ → $S_2^+ + H_2$<br>→ $S_2H^+ + H$<br>→ $H_2S^+ + S$ | <br><br>+9 | 0.75<br>0.25<br>0 | 8.2e-10<br>8.2e-10 | 1.77<br>1.77 | 1.4<br>1.4 | 0<br>0 | Capture rate theory, Ionpol1-2 ($T_m$ = 233 K). See also (Anicich 2003). |
| 147. | $S + H_3^+$ → $HS^+ + H_2$<br>→ $H + H_2S^+$ | -240<br>-180 | 2.0e-9<br>0.4e-9 | 0<br>0 | 0<br>0 | 3<br>3 | 0<br>0 | Capture rate theory, close to $O + H_3^+$ (Milligan & McEwan 2000) |
| 148. | $S + HCO^+$ → $HS^+ + CO$ | -72 | 3.30e-10 | 0 | 0 | 2 | 0 | KIDA |
| 149. | $S + N_2H^+$ → $HS^+ + N_2$ | | 1.1e-9 | 0 | 0 | 2 | 0 | KIDA |
| 150. | $S + CH^+$ → $H + CS^+$<br>→ $C + HS^+$<br>→ $CH + S^+$ | -310<br>-38<br>-27 | 4.7e-10<br>4.7e-10<br>4.7e-10 | 0<br>0<br>0 | 0<br>0<br>0 | 2<br>2<br>2 | 0<br>0<br>0 | KIDA |
| 151. | $S + CH_3^+$ → $H_2 + HCS^+$<br>→ $H_2CS^+ + H$ | -357<br>-132 | 1.40e-9<br>0 | 0 | 0 | 2 | 0 | KIDA |
| 152. | $S + CH_5^+$ → $HS^+ + CH_4$ | | 1.30e-9 | 0 | 0 | 2 | 0 | KIDA |
| 153. | $S + C_2H_2^+$ → $S^+ + C_2H_2$<br>→ $H + HC_2S^+$ | -100<br>-34 | 5.0e-10<br>5.0e-10 | 0<br>0 | 0<br>0 | 3<br>3 | 0<br>0 | Capture rate theory |
| 154. | $S + C_2H_3^+$ → $H_2 + HC_2S^+$<br>→ $H + H_2C_2S^+$<br>→ $CH_3^+ + CS$ | -165<br>-130<br>-17 | 0<br>1.0e-9<br>0 | <br>0 | <br>0 | <br>3 | <br>0 | Capture rate theory |
| 155. | $S + C_2H_4^+$ → $H + H_2 + HC_2S^+$<br>→ $CH_3 + HCS^+$<br>→ $CH_3^+ + HCS$<br>→ $C_2H_3^+ + HS$<br>→ $H + CH_3CS^+$<br>→ $H_2 + H_2C_2S^+$ | +231<br>-145<br>+63<br>-56<br>-213<br>-266 | 0<br>1.0e-10<br>0<br>0<br>1.0e-10<br>1.0e-10 | <br>0<br><br><br><br>0 | <br>0<br><br><br><br>0 | <br>3<br><br><br><br>3 | <br>0<br><br><br><br>0 | By comparison with $O + C_2H_4^+$(Anicich 2003). Branching ratio deduced from exothermicities. |
| 156. | $S + c\text{-}C_3H_2^+$ → $H + HC_3S^+$<br>→ $C_2H + HCS^+$ | -225<br>-41 | 1.0e-9<br>0 | 0 | 0 | 3 | 0 | KIDA |
| 157. | $S + l\text{-}C_3H_2^+$ → $H + HC_3S^+$<br>→ $C_2H + HCS^+$ | | 1.0e-9<br>0 | 0 | 0 | 3 | 0 | KIDA |
| 158. | $S + t\text{-}C_3H_2^+$ → $H + HC_3S^+$ | | 1.0e-9 | 0 | 0 | 3 | 0 | KIDA |

| | | | | | | | | |
|---|---|---|---|---|---|---|---|---|
| | → $C_2H + HCS^+$ | | 0 | | | | | |
| 159. | $S + c\text{-}C_3H_3^+$ → $H_2 + HC_3S^+$<br>→ $H + H_2C_3S^+$<br>→ $CS + C_2H_3^+$<br>→ $HCS^+ + C_2H_2$ | -132<br>+49<br>+94<br>-63 | 1.0e-10<br>0<br>0<br>4.0e-10 | 0<br><br><br>0 | 0<br><br><br>0 | 4<br><br><br>4 | 0<br><br><br>0 | See appendix A |
| 160. | $S + l\text{-}C_3H_3^+$ → $H_2 + HC_3S^+$<br>→ $H + H_2C_3S^+$<br>→ $CS + C_2H_3^+$<br>→ $HCS^+ + C_2H_2$ | -272<br>-91<br>-45<br>-112 | 1.0e-10<br>2.0e-10<br>0<br>2.0e-10 | 0<br>0<br><br>0 | 0<br>0<br><br>0 | 4<br>4<br><br>4 | 0<br>0<br><br>0 | See appendix A |
| 161. | $S + CH$ → $CS + H$ | -345 | 1.4e-10 | 0 | 0 | 3 | 0 | Capture rate theory |
| 162. | $S + CH_2$ → $HCS + H$<br>→ $CS + H_2$ | -150<br>-387 | 1.4e-10<br>0 | 0 | 0 | 2 | 0 | Capture rate theory. We neglect the $CS + H_2$ exit channel assuming that the TS for $H_2$ elimination is close to 350 kJ/mol by comparison with $O + CH_2$ (Zhang *et al.* 2004). |
| 163. | $S + CH_3$ → $H_2CS + H$ | -81 | 1.4e-10 | 0 | 0 | 2 | 0 | KIDA |
| 164. | $S + C_2$ → $CS + C$ | -212 | 2.0e-10 | 0 | 0 | 2 | 0 | Capture rate theory |
| 165. | $S + C_2H$ → $C_2S + H$<br>→ $CS + CH$ | -20<br>+27 | 1.0e-10 | 0 | 0 | 3 | 0 | Capture rate theory |
| 166. | $S + C_2H_3$ → $H + H_2CCS$<br>→ $CH_3 + CS$<br>→ $SH + C_2H_2$ | -160<br>-131<br>-200 | 6.0e-11<br>4.0e-11<br>1.0e-11 | 0<br>0<br>0 | 0<br>0<br>0 | 2<br>2<br>3 | 0<br>0<br>0 | Capture rate theory leading to the two first exit channel. Direct H atom abstraction, leading to SH + $C_2H_2$, is supposed to be a minor reaction. |
| 167. | $S + l\text{-}C_3H$ → $CS + C_2H$<br>→ $C_3S + H$ | -167<br>-221 | 7.0e-11<br>3.0e-11 | 0<br>0 | 0<br>0 | 2<br>2 | 0<br>0 | (Flores *et al.* 2001, Flores *et al.* 2002) |
| 168. | $S + c\text{-}C_3H$ → $CS + C_2H$<br>→ $C_3S + H$ | -154<br>-208 | 5.0e-11<br>5.0e-11 | 0<br>0 | 0<br>0 | 2<br>2 | 0<br>0 | (Flores et al. 2002) |
| 169. | $S + l,t\text{-}C_3H_2$ → $C_2H_2 + CS$<br>→ $C_2H_2 + CS$<br>→ $HC_3S + H$ | -307<br>+73<br>-130 | 1.0e-10<br>0<br>1.0e-10 | 0<br>0<br>0 | 0<br>0<br>0 | 3<br>0<br>3 | 0<br>0<br>0 | Capture rate theory |
| 170. | $S + c\text{-}C_3H_2$ → $C_2H_2 + CS$<br>→ $C_2H_2 + CS$<br>→ $HC_3S + H$ | -224<br>+156<br>-47 | 1.0e-10<br>0<br>1.0e-10 | 0<br><br>0 | 0<br><br>0 | 3<br><br>3 | 0<br><br>0 | See appendix A |
| 171. | $S + C_4$ → $C_3 + CS$ | -220 | 1.0e-10 | 0 | 0 | 3 | 0 | Capture rate theory |
| 172. | $S + C_4H$ → $CS + l\text{-}C_3H$<br>→ $C_4S + H$ | -50<br>-69 | 5.0e-11<br>5.0e-11 | 0<br>0 | 0<br>0 | 2<br>2 | 0<br>0 | Capture rate theory |
| 173. | $S + C_6$ → $C_5 + CS$ | -229 | 1.0e-10 | 0 | 0 | 3 | 0 | Capture rate theory |

| | | | | | | | | |
|---|---|---|---|---|---|---|---|---|
| 174. | S + $C_2N$ → CS + CN | -251 | 7.0e-11 | 0.17 | 0 | 3 | 0 | Capture rate theory |
| 175. | S + $H_2CN$ → SH + HCN<br>→ SH + HNC<br>→ H + HCNS | -243<br>-190<br>-31 | 3.0e-11<br>0<br>3.0e-11 | 0<br>0<br>0 | 0<br>0<br>0 | 3<br>3<br>3 | 0<br>0<br>0 | Radical-radical reaction leading to direct H atom abstraction and H + HCNS through $H_2CNS$ formation. |
| 176. | S + $C_3N$ → CS + $C_2N$<br>→ $C_2S$ + CN | -12<br>+38 | 1.0e-10<br>0 | 0 | 0 | 10 | 0 | Capture rate theory |
| 177. | S + $C_4N$ → CS + $C_3N$ | -150 | 7.0e-11 | 0.17 | 0 | 3 | 0 | Capture rate theory |
| 178. | S + $C_2S$ → CS + CS | -325 | 1.0e-10 | 0 | 0 | 3 | 0 | Capture rate theory |
| 179. | S + NH → NS + H | -116 | 1.0e-10 | 0 | 0 | 3 | 0 | Capture rate theory |
| 180. | S + $NH_2$ → NS + $H_2$<br>→ HNS + H | -167<br>-1 | "0" | | | | | HNS + H exit channel may be endothermic and NS + $H_2$ may involve high exit transition state. Back dissociation of the $H_2NS$ complex, first step of the reaction, is then likely favored and we neglect this reaction. |
| 181. | S + OH → SO + H | -82 | 6.6e-11 | 0 | 0 | 3 | 0 | (Jourdain et al. 1979) |
| 182. | S + $H_2O^+$ → $SO^+$ + $H_2$<br>→ O + $H_2S^+$<br>→ $HS^+$ + OH<br>→ H + $HSO^+$<br>→ $S^+$ + $H_2O$ | -254<br>-15<br>-68<br>-81<br>-217 | 4.0e-10<br>0<br>4.0e-10<br>0<br>2.0e-10 | 0<br>0<br>0<br>0<br>0 | 0<br>0<br>0<br>0<br>0 | 3<br>3<br>3<br>3<br>3 | 0<br>0<br>0<br>0<br>0 | Capture rate theory |
| 183. | S + $O_2$ → SO + O | -22 | 2.0e-12 | -0.6 | 0 | 1.4 | 10 | The rate constant has been measured in the 298–878 K (Lu *et al.* 2004). |
| 184. | S + $CO^+$ → CO + $S^+$ | -352 | 1.1e-9 | 0 | 0 | 2 | 0 | KIDA |
| 185. | S + HCO → H + OCS<br>→ SH + CO | -246<br>-288 | 8.0e-11<br>4.0e-11 | 0<br>0 | 0<br>0 | 2<br>2 | 10<br>10 | (Loison *et al.* 2012) |
| 186. | S + CCO → CO + CS<br>→ C + OCS | -449<br>-62 | 1.0e-10<br>0 | 0 | 0 | 2 | 10 | (Loison et al. 2012) |
| 187. | S + $C_4S$ → $C_3S$ + CS | -182 | 1.0e-10 | 0 | 0 | 3 | 0 | Capture rate theory |
| 188. | S + $CH_3O$ → $CH_3$ + SO | -128 | 4.0e-11 | 0 | 0 | 2 | 0 | Capture rate theory, similar to the O + $CH_3O$ reaction (Ewig et al. 1987) |
| 189. | S + $CH_2OH$ → $H_2CO$ + HS<br>→ $H_2CS$ + OH | -222<br>-92 | 4.0e-11<br>4.0e-11 | 0<br>0 | 0<br>0 | 2<br>2 | 0<br>0 | Capture rate theory, similar to the O + $CH_2OH$ reaction (Grotheer et al. 1989) |
| | | | | | | | | |
| 190. | $HS^+$ + $H_2O$ → S + $H_3O^+$ | -27 | 1 | 8.5e-10 | 5.41 | 2 | 0 | KIDA |
| 191. | $HS^+$ + HNC → $HNCS^+$ + H<br>→ $HSCN^+$ + H | -35<br>+104 | 0.1<br>0 | 1.04e-9<br>1.04e-9 | 6.41<br>6.41 | 3<br>3 | 0<br>0 | Capture rate theory, Ionpol1 ($T_m$ = 800 K). |

| | | | | | | | | |
|---|---|---|---|---|---|---|---|---|
| | → $HCNH^+ + S$ | -102 | 0.9 | 1.04e-9 | 6.41 | 3 | 0 | |
| 192. | $HS^+ + HCN$ → $HNCS^+ + H$<br>→ $HCNH^+ + S$ | +18<br>-49 | 0<br>1.0 | <br>9.53e-10 | <br>6.62 | <br>3 | <br>0 | Capture rate theory, Ionpol1 ($T_m$ = 800 K). |
| 193. | $H_2S^+ + HNC$ → $HNCSH^+ + H$<br>→ $HCNH^+ + SH$<br>→ $H_3S^+ + CN$ | -35<br>-84<br>+92 | 0.1<br>0.9<br>0 | 9.97e-10<br>9.97e-10 | 6.41<br>6.41 | 3<br>3 | 0<br>0 | Capture rate theory, Ionpol1 ($T_m$ = 800 K). |
| 194. | $H_2S^+ + HCN$ → $HCNH^+ + SH$ | -31 | 1.0 | 9.46e-10 | 6.62 | 3 | 0 | Capture rate theory, Ionpol1 ($T_m$ = 800 K). |
| 195. | $H_2S + H_3^+$ → $H_2 + H_3S^+$ | | 1 | 2.67e-9 | 1.77 | 2 | 0 | KIDA |
| 196. | $H_2S + H_3O^+$ → $H_2O + H_3S^+$ | | 1 | 1.27e-9 | 1.77 | 2 | 0 | KIDA |
| 197. | $H_2S + HCO^+$ → $CO + H_3S^+$ | | 1 | 1.12e-9 | 1.77 | 2 | 0 | KIDA |
| 198. | $CO + HSO^+$ → $SO + HCO^+$ | -13 | 1.0e-9 | 0 | 0 | 2 | 0 | Capture rate theory, exothermicities from (Hunter & Lias 1998, Cheng *et al.* 1997) |
| 199. | $H_2O + HSO^+$ → $SO + H_3O^+$ | -79 | 2.0e-9 | 0 | 0 | 2 | 0 | Capture rate theory |
| 200. | $SO + H_3^+$ → $H_2 + HSO^+$ | -159 | 1.0 | 2.58e-9 | 2.93 | 2 | 0 | KIDA |
| 201. | $SO + HCO^+$ → $CO + HSO^+$ | +13 | 1.0e-9 | 0 | 1500 | 2 | 1000 | Using (Hunter & Lias 1998) and (Cheng et al. 1997) |
| 202. | $C_3S + H_3^+$ → $HC_3S^+ + H_2$ | | 1.0 | 4.29e-9 | 4.39 | 2 | 0 | Capture rate theory, Ionpol1 ($T_m$ = 800 K). |
| 203. | $C_3S + H_3O^+$ → $HC_3S^+ + H_2O$ | | 1.0 | 1.88e-9 | 4.39 | 2 | 0 | Capture rate theory, Ionpol1 ($T_m$ = 800 K). |
| 204. | $C_3S + HCO^+$ → $HC_3S^+ + CO$ | | 1.0 | 1.61e-9 | 4.39 | 2 | 0 | Capture rate theory, Ionpol1 ($T_m$ = 800 K). |
| 205. | $CH_3SH + H_3^+$ → $H_2 + CH_3SH_2^+$ | | 1 | 3.2e-9 | 2.3 | 3 | 0 | Capture rate theory, Ionpol1-2 ($T_m$ = 407 K). |
| 206. | $CH_3SH + H_3O^+$ → $H_2O + CH_3SH_2^+$ | | 1 | 1.5e-9 | 2.3 | 3 | 0 | Capture rate theory, Ionpol1-2 ($T_m$ = 407 K). |
| 207. | $CH_3SH + HCO^+$ → $CO + CH_3SH_2^+$ | | 1 | 1.3e-9 | 2.3 | 3 | 0 | Capture rate theory, Ionpol1-2 ($T_m$ = 407 K). |
| 208. | $HNCS + H_3^+$ → $H_2NCS^+ + H_2$<br>→ $HNCSH^+ + H_2$ | | 0.50<br>0.50 | 3.47e-9<br>3.47e-9 | 2.92<br>2.92 | 3<br>3 | 0<br>0 | KIDA, Ionpol1-2 ($T_m$ = 638 K). (Gronowski & Kolos 2014) |
| 209. | $HSCN + H_3^+$ → $H_2SCN^+ + H_2$<br>→ $HNCSH^+ + H_2$ | | 0.50<br>0.50 | 3.20e-9<br>3.20e-9 | 5.17<br>5.17 | 3<br>3 | 0<br>0 | KIDA, Ionpol1 ($T_m$ = 2005 K). (Gronowski & Kolos 2014) |
| 210. | $HCNS + H_3^+$ → $H_2CNS^+ + H_2$<br>→ $HCNSH^+ + H_2$ | | 0.50<br>0.50 | 3.10e-9<br>3.10e-9 | 5.45<br>5.45 | 3<br>3 | 0<br>0 | Capture rate theory, Ionpol1 ($T_m$ = 2075 K). ($T_m$ = 2075 K). |
| 211. | $HNCS + HCO^+$ → $H_2NCS^+ + CO$<br>→ $HNCSH^+ + CO$ | | 0.50<br>0.50 | 1.32e-9<br>1.32e-9 | 2.92<br>2.92 | 3<br>3 | 0<br>0 | KIDA, Ionpol1-2 ($T_m$ = 638 K). (Gronowski & Kolos 2014) |
| 212. | $HSCN + HCO^+$ → $H_2SCN^+ + CO$<br>→ $HNCSH^+ + CO$ | ≈0 | 0<br>1.00 | 1.18e-9<br>1.18e-9 | 5.17<br>5.17 | 3<br>3 | 0<br>0 | KIDA, Ionpol1 ($T_m$ = 2005 K). (Gronowski & Kolos 2014) |
| 213. | $HCNS + HCO^+$ → $H_2CNS^+ + CO$<br>→ $HCNSH^+ + CO$ | | 0.50<br>0.50 | 1.22e-9<br>1.22e-9 | 5.45<br>5.45 | 3<br>3 | 0<br>0 | Capture rate theory, Ionpol1 ($T_m$ = 2075 K). |
| 214. | $H_2CCS + H_3^+$ → $CH_3CS^+ + H_2$ | | 1.0 | 2.90e-9 | 2.39 | 3 | 0 | Capture rate theory, Ionpol1-2 ($T_m$ = 145 K). |

| | | | | | | | | |
|---|---|---|---|---|---|---|---|---|
| 215. | $H_2CCS + HCO^+ \rightarrow CH_3CS^+ + CO$ | | 1.0 | 1.17e-9 | 2.39 | 3 | 0 | Capture rate theory, Ionpol1-2 ($T_m$ = 145 K). |
| 216. | $NH_2CHS + H_3^+ \rightarrow NH_2CHSH^+ + H_2$<br>$\rightarrow NH_3CHS^+ + H_2$<br>$\rightarrow NH_3 + HCS^+ + H_2$ | -415<br>-327<br>-158 | 1.0<br>0<br>0 | 3.68e-9 | 5.6 | 3 | 0 | Capture rate theory, Ionpol1 ($T_m$ = 2075 K). We merge $NH_2CHSH^+$ and $NH_3CHS^+$. |
| 217. | $NH_2CHS + HCO^+ \rightarrow NH_2CHSH^+ + CO$ | -267 | 1.0 | 1.40e-9 | 5.6 | 3 | 0 | Capture rate theory, Ionpol1 ($T_m$ = 2075 K). |
| 218. | $NH_2CH_2SH + H_3^+ \rightarrow NH_3CH_2SH^+ + H_2$ | -437 | 1.0 | 3.66e-9 | 1.4 | 3 | 0 | Capture rate theory, Ionpol1-2 ($T_m$ = 142 K). |
| 219. | $NH_2CH_2SH + HCO^+ \rightarrow NH_3CH_2SH^+ + CO$ | -289 | 1.0 | 1.39e-9 | 1.4 | 3 | 0 | Capture rate theory, Ionpol1-2 ($T_m$ = 142 K). |
| | | | | | | | | |
| 220. | $S^+ + e^- \rightarrow S + h\nu$ | | 3.9e-12 | -0.63 | 0 | 2 | 0 | KIDA |
| 221. | $HS^+ + e^- \rightarrow H + S$ | | 2.0e-7 | -0.5 | 0 | 2 | 0 | KIDA |
| 222. | $H_2S^+ + e^- \rightarrow H + HS$<br>$\rightarrow H + H + S$<br>$\rightarrow H_2S + h\nu$ | -632<br>-277<br>-1009 | 1.5e-7<br>1.5e-7<br>1.1e-10 | -0.5<br>-0.5<br>-0.7 | 0<br>0<br>0 | 2<br>2<br>100 | 0<br>0<br>0 | KIDA. The reference for the $H_2S^+ + e^- \rightarrow H_2S + h\nu$ reaction is unknown. This rate is highly uncertain. |
| 223. | $H_3S^+ + e^- \rightarrow H + H_2S$<br>$\rightarrow H_2 + HS$<br>$\rightarrow H + H + HS$<br>$\rightarrow H + H_2 + S$ | -608<br>-592<br>-231<br>-310 | 4.8e-8<br>4.2e-8<br>1.6e-7<br>2.8e-8 | -0.86<br>-0.86<br>-0.86<br>-0.86 | 0<br>0<br>0<br>0 | 1.6<br>1.6<br>1.6<br>1.6 | 3<br>3<br>3<br>3 | (Kaminska *et al.* 2008) |
| 224. | $HSO^+ + e^- \rightarrow H + SO$<br>$\rightarrow HS + O$<br>$\rightarrow H + S + O$ | -732<br>-566<br>-211 | 1.0e-7<br>5.0e-8<br>5.0e-8 | -0.5<br>-0.5<br>-0.5 | 0<br>0<br>0 | 2<br>2<br>2 | 0<br>0<br>0 | Capture rate theory |
| 225. | $HCS^+ + e^- \rightarrow S + CH$<br>$\rightarrow H + CS$<br>$\rightarrow H + C + S$ | -142<br>-518<br>+196 | 7.86e-7<br>1.84e-7<br>0 | -0.57<br>-0.57 | 0<br>0 | 1.6<br>1.6 | 0<br>0 | (Montaigne *et al.* 2005) |
| 226. | $H_3CS^+ + e^- \rightarrow H + H_2CS$<br>$\rightarrow H + H + HCS$<br>$\rightarrow H + H_2 + CS$<br>$\rightarrow CH_2 + SH$<br>$\rightarrow H_2S + CH$ | -553<br>-154<br>-391<br>-359<br>-313 | 2.2e-7<br>2.2e-7<br>2.2e-7<br>3.8e-8<br>1.5e-8 | -0.78<br>-0.78<br>-0.78<br>-0.78<br>-0.78 | 0<br>0<br>0<br>0<br>0 | 2<br>2<br>2<br>2<br>2 | 0<br>0<br>0<br>0<br>0 | Equal to $CH_2OH^+ + e^-$ (Hamberg *et al.* 2007). |
| 227. | $CH_3SH_2^+ + e^- \rightarrow CH_3 + H_2S$<br>$\rightarrow CH_3 + SH + H$<br>$\rightarrow CH_2 + H + H_2S$<br>$\rightarrow CH_3SH + H$<br>$\rightarrow CH_3S + H_2$<br>$\rightarrow H_2CS + H_2 + H$ | | 8.0e-8<br>4.5e-7<br>1.9e-7<br>2.7e-8<br>5.3e-8<br>5.9e-8 | -0.59<br>-0.59<br>-0.59<br>-0.59<br>-0.59<br>-0.59 | 0<br>0<br>0<br>0<br>0<br>0 | 1.4<br>1.4<br>1.4<br>1.4<br>1.4<br>1.4 | 0<br>0<br>0<br>0<br>0<br>0 | Equal to $CH_3OH_2^+ + e^-$ (Geppert *et al.* 2006) |
| 228. | $HC_2S^+ + e^- \rightarrow H + C_2S$ | -562 | 1.5e-7 | -0.5 | 0 | 3 | 0 | Methodology described in appendix A. |

| | | | | | | | | | |
|---|---|---|---|---|---|---|---|---|---|
| | | → $CH + CS$ | -455 | 7.5e-8 | -0.5 | 0 | 3 | 0 | |
| | | → $C_2H + S$ | -509 | 7.5e-8 | -0.5 | 0 | 3 | 0 | |
| 229. | $H_2C_2S^+ + e^-$ | → $H + HCCS$ | -486 | 1.5e-7 | -0.5 | 0 | 3 | 0 | Methodology described in appendix A. |
| | | → $H + H + C_2S$ | -64 | 1.0e-8 | -0.5 | 0 | 3 | 0 | |
| | | → $CH_2 + CS$ | -387 | 1.5e-7 | -0.5 | 0 | 3 | 0 | |
| 230. | $CH_3CS^+ + e^-$ | → $H + H_2CCS$ | | 1.5e-7 | -0.5 | 0 | 3 | 0 | Methodology described in appendix A. |
| | | → $CH_3 + CS$ | | 1.5e-7 | -0.5 | 0 | 3 | 0 | |
| 231. | $NH_3CHS^+ + e^-$ | → $NH_3 + CS + H$ | | 2.0e-7 | -0.5 | 0 | 3 | 0 | Methodology described in appendix A. |
| | | → $H + NH_2CHS$ | | 1.0e-7 | -0.5 | 0 | 3 | 0 | |
| | | → $H_2S + HCN + H$ | | 1.0e-7 | -0.5 | 0 | 3 | 0 | |
| 232. | $HC_3S^+ + e^-$ | → $H + C_3S$ | -447 | 1.0e-7 | -0.5 | 0 | 3 | 0 | Methodology described in appendix A. |
| | | → $C_2H + CS$ | -385 | 1.0e-7 | -0.5 | 0 | 3 | 0 | |
| | | → $CH + C_2S$ | -27 | 1.0e-7 | -0.5 | 0 | 4 | 0 | |
| 233. | $H_2C_3S^+ + e^-$ | → $H + HC_3S$ | -462 | 1.0e-7 | -0.5 | 0 | 3 | 0 | Methodology described in appendix A. |
| | | → $CH_2 + C_2S$ | -216 | 1.0e-7 | -0.5 | 0 | 3 | 0 | |
| | | → $C_2H_2 + CS$ | -638 | 1.0e-7 | -0.5 | 0 | 3 | 0 | |
| 234. | $HC_4S^+ + e^-$ | → $H + C_4S$ | -466 | 1.0e-7 | -0.5 | 0 | 4 | 0 | Methodology described in appendix A. |
| | | → $CH + C_3S$ | -284 | 1.0e-7 | -0.5 | 0 | 4 | 0 | |
| | | → $C_2H + C_2S$ | -331 | 1.0e-7 | -0.5 | 0 | 4 | 0 | |
| | | → l-$C_3H + CS$ | -447 | 1.0e-7 | -0.5 | 0 | 4 | 0 | |
| | | → $C_4H + S$ | -396 | 1.0e-7 | -0.5 | 0 | 4 | 0 | |
| 235. | $HNCS^+ + e^-$ | → $HNC + S$ | -619 | 1.0e-7 | -0.5 | 0 | 3 | 0 | Methodology described in appendix A. |
| | | → $HCN + S$ | -671 | 5.0e-7 | -0.5 | 0 | 3 | 0 | |
| | | → $NH + CS$ | -430 | 1.5e-7 | -0.5 | 0 | 3 | 0 | |
| 236. | $HCNS^+ + e^-$ | → $S + HCN$ | -740 | 1.5e-7 | -0.5 | 0 | 3 | 0 | Methodology described in appendix A. |
| | | → $CH + NS$ | -255 | 1.5e-7 | -0.5 | 0 | 3 | 0 | |
| 237. | $HSCN^+ + e^-$ | → $HS + CN$ | -808 | 1.5e-7 | -0.5 | 0 | 3 | 0 | Methodology described in appendix A. |
| | | → $S + HCN$ | -622 | 1.5e-7 | -0.5 | 0 | 3 | 0 | |
| 238. | $H_2NCS^+ + e^-$ | → $HNCS + H$ | -550 | 1.7e-7 | -0.5 | 0 | 3 | 0 | Methodology described in appendix A. We consider 50% of H elimination leading to energized HNCS**. As the HNCS → HSCN isomerization TS is 270 kJ/mol, we consider than most of the HNCS is produced above the isomerization TS in a similar way than HCN in the DR of $HCNH^+$ (Mendes *et al.* 2012). The HNCS** produced above the isomerization TS leads to |
| | | → $HSCN + H$ | -514 | 1.3e-7 | -0.5 | 0 | 3 | 0 | |
| | | → $NH_2 + CS$ | -403 | 3.0e-7 | -0.5 | 0 | 3 | 0 | |

| | | | | | | | | |
|---|---|---|---|---|---|---|---|---|
| | | | | | | | | similar HNCS or HSCN production as the ro-vibrational densities of both isomers are similar at the TS energy (see appendix A). |
| 239. | $HNCSH^+ + e^-$ → HNCS + H<br>→ HSCN + H<br>→ HNC + SH<br>→ HCN + SH | -587<br>-549<br>-598<br>-651 | 1.5e-7<br>1.5e-7<br>1.5e-7<br>1.5e-7 | -0.5<br>-0.5<br>-0.5<br>-0.5 | 0<br>0<br>0<br>0 | 3<br>3<br>3<br>3 | 0<br>0<br>0<br>0 | Similar reasons than for $H_2NCS^+ + e^-$ |
| 240. | $H_2SCN^+ + e^-$ → HSCN + H<br>→ HNCS + H<br>→ $H_2S$ + CN<br>→ H + SH + CN | -719<br>-759<br>-656<br>-287 | 1.6e-7<br>1.4e-7<br>2.0e-7<br>2.0e-7 | -0.5<br>-0.5<br>-0.5<br>-0.5 | 0<br>0<br>0<br>0 | 3<br>3<br>3<br>3 | 0<br>3<br>0<br>0 | Similar reasons than for $H_2NCS^+ + e^-$ |
| 241. | $H_2CNS^+ + e^-$ → HCNS + H<br>→ $CH_2$ + NS<br>→ H + HCN + S | -563<br>-370<br>-428 | 1.0e-7<br>3.0e-7<br>2.0e-7 | -0.5<br>-0.5<br>-0.5 | 0<br>0<br>0 | 3<br>3<br>3 | 0<br>0<br>0 | Methodology described in appendix A. We consider 50% of H elimination, most of the HCNS** will dissociate. |
| 242. | $HCNSH^+ + e^-$ → HCNS + H<br>→ HCN + SH<br>→ H + CN + SH | -517<br>-728<br>-194 | 1.0e-7<br>3.0e-7<br>2.0e-7 | -0.5<br>-0.5<br>-0.5 | 0<br>0<br>0 | 3<br>3<br>3 | 0<br>0<br>0 | Methodology described in appendix A. We consider 50% of H elimination, most of the HCNS** and HSNC** will dissociate. |
| 243. | $NH_2CHSH^+ + e^-$ → $NH_2CHS$ + H<br>→ $NH_2$ + $H_2CS$<br>→ $NH_3$ + HCS<br>→ $NH_3$ + H + CS | -467<br>-424<br>-483<br>-272 | 1.5e-7<br>1.5e-7<br>1.5e-7<br>1.5e-7 | -0.5<br>-0.5<br>-0.5<br>-0.5 | 0<br>0<br>0<br>0 | 3<br>3<br>3<br>3 | 0<br>0<br>0<br>0 | Methodology described in appendix A. |
| 244. | $NH_3CH_2SH^+ + e^-$ → $NH_2CH_2SH$ + H<br>→ $NH_3$ + $CH_2SH$<br>→ $NH_3$ + $H_2CS$ + H | -445<br>-547<br>-366 | 1.0e-7<br>1.0e-7<br>4.0e-7 | -0.5<br>-0.5<br>-0.5 | 0<br>0<br>0 | 3<br>3<br>3 | 0<br>0<br>0 | Methodology described in appendix A. |
| | | | | | | | | |
| 245. | C + s-$H_2S$ → s-$H_2CS$ | | 1.0 | 0 | 0 | 1 | 0 | Eley-Rideal mechanism (Ruaud *et al.* 2015) |
| 246. | s-H + s-S → s-HS | | 1.0 | 0 | 0 | 1 | 0 | Methodology described in appendix A. |
| 247. | s-H + s-HS → s-$H_2S$ | | 1.0 | 0 | 0 | 1 | 0 | Methodology described in appendix A. |
| 248. | s-H + s-$H_2S$ → s-$H_2$ + s-HS | | 1.0 | 0 | 860 | 1 | 400 | From gas phase study. Activation barrier is estimated to 860 K in the 190-464 K range (Kurylo et al. 1971) and to 1350 K in the 298-598 K range (Peng et al. 1999). |
| 249. | s-H + s-CS → s-HCS | | 1.0 | 0 | 1000 | 1 | 400 | Theoretical gas phase value, see appendix A |
| 250. | s-H + s-HCS → s-$H_2CS$<br>→ s-$H_2$ + s-CS | | 1.0<br>0 | 0 | 0 | 1 | 0 | Methodology described in appendix A. |
| 251. | s-H + s-$H_2CS$ → s-$CH_3S$ | -216 | 0.5 | 0 | 1200 | 1 | 200 | Theoretical gas phase value, see appendix A |

| | | | | | | | | |
|---|---|---|---|---|---|---|---|---|
| | → s-$CH_2SH$<br>→ s-$H_2$ + s-HCS | -180<br>-45 | 0.5<br>0 | 0 | 800 | 1 | 200 | |
| 252. | s-H + s-$CH_3S$ → s-$CH_3SH$ | | 1.0 | 0 | 0 | 1 | 0 | Methodology described in appendix A. |
| 253. | s-H + s-$CH_2SH$ → s-$CH_3SH$ | | 1.0 | 0 | 0 | 1 | 0 | Methodology described in appendix A. |
| 254. | s-H + s-$CH_3SH$ → s-$CH_2SH$ + s-$H_2$<br>→ s-$CH_3S$ + s-$H_2$<br>→ s-$CH_3$ + s-$H_2S$ | | 0<br>0.5<br>0.5 | <br>0<br>0 | <br>800<br>1600 | <br>1.4<br>1.6 | <br>200<br>400 | By comparison with the gas phase (Kerr *et al.* 2015, Martin *et al.* 1988) |
| 255. | s-H + s-HNCS → s-$NH_2CS$<br>→ s-HNCSH<br>→ s-HNCHS<br>→ s-HNC + s-SH | -115<br>-54<br>-98<br>-12 | 0.4<br>0.4<br>0.2<br>0 | 0<br>0<br>0<br>0 | 3600<br>2600<br>5400<br>2600 | 1<br>1<br>1<br>1 | 1000<br>1000<br>1000<br>1000 | Theoretical gas phase value, see appendix A |
| 256. | s-H + s-HSCN → s-HSCHN<br>→ s-HNCSH<br>→ s-HCN + s-SH<br>→ s-HNC + s-SH<br>→ s-$H_2S$ + s-CN | -108<br>-93<br>-103<br>-50<br>+51 | 0.3<br>0.5<br>0.2<br>0<br>0 | 0<br>0<br>0<br>0 | 4000<br>4000<br>4000<br>4000 | 1<br>1<br>1<br>1 | 1000<br>1000<br>1000<br>1000 | Theoretical gas phase value, see appendix A |
| 257. | s-H + s-$NH_2CS$ → s-$NH_2CHS$<br>→ s-$H_2$ + s-HNCS | -378<br>-311 | 0.6<br>0.4 | 0<br>0 | 0<br>0 | 2<br>2 | 0<br>0 | Methodology described in appendix A. |
| 258. | s-H + s-HNCSH → s-HNCHSH<br>→ s-HNCS + s-$H_2$<br>→ s-HSCN + s-$H_2$ | -398<br>-371<br>-333 | 0.6<br>0.3<br>0.1 | 0<br>0<br>0 | 0<br>0<br>0 | 2<br>2<br>2 | 0<br>0<br>0 | Methodology described in appendix A. |
| 259. | s-H + s-HNCHS → s-$NH_2CHS$<br>→ s-HNCHSH<br>→ s-HNCS + s-$H_2$ | -396<br>-355<br>-328 | 0.3<br>0.3<br>0.4 | 0<br>0<br>0 | 0<br>0<br>0 | 2<br>2<br>2 | 0<br>0<br>0 | Methodology described in appendix A. |
| 260. | s-H + s-HSCHN → s-HNCHSH<br>→ s-HSCN + s-$H_2$ | -383<br>-317 | 0.6<br>0.4 | 0<br>0 | 0<br>0 | 2<br>2 | 0<br>0 | Methodology described in appendix A. |
| 261. | s-H + s-$NH_2CHS$ → s-$NH_2CH_2S$ | | 1 | 0 | 1000 | 2 | 600 | Same as H + $H_2CS$ reaction |
| 262. | s-H + s-HNCHSH → s-$NH_2CHSH$ | | 1 | 0 | 1000 | 2 | 600 | Same as H + $H_2CS$ reaction |
| 263. | s-H + s-$NH_2CH_2S$ → s-$NH_2CH_2SH$ | | 1 | 0 | 0 | 2 | 0 | Methodology described in appendix A. |
| 264. | s-H + s-$NH_2CHSH$ → s-$NH_2CH_2SH$ | | 1 | 0 | 0 | 2 | 0 | Methodology described in appendix A. |
| 265. | s-H + s-SO → s-HSO | -236 | 1 | 0 | 0 | 1 | 0 | We supposed no barrier for H addition by comparison with H + $O_2$ reaction. |
| 266. | s-H + s-HSO → s-HSOH<br>→ s-$H_2SO$<br>→ s-HS + s-OH | -317<br>-221<br>-31 | 0<br>0<br>1.0 | <br><br>0 | <br><br>0 | <br><br>1 | <br><br>0 | Methodology described in appendix A. Some HSOH, $H_2SO$ as well as S + $H_2O$ and $H_2$ + SO may also be produced. |

| | | | | | | | | |
|---|---|---|---|---|---|---|---|---|
| | → s-$H_2$ + s-SO<br>→ s-HS + s-$H_2O$<br>→ s-O + s-$H_2S$ | -190<br>-169<br>+23 | 0<br>0<br>0 | | | | | |
| 267. | s-H + s-$C_2S$ → s-HCCS | | 1.0 | 0 | 0 | 1 | 0 | Methodology described in appendix A. |
| 268. | s-H + s-HCCS → s-$H_2CCS$ | | 1.0 | 0 | 0 | 1 | 0 | Methodology described in appendix A. |
| 269. | s-H + s-$C_3S$ → s-$HC_3S$ | | 1.0 | 0 | 800 | 1 | 400 | Theoretical gas phase value, see appendix A |
| 270. | s-H + s-$HC_3S$ → s-$H_2C_3S$ | | 1.0 | 0 | 0 | 1 | 0 | Methodology described in appendix A. We consider only one $H_2C_3S$ isomer. |
| 271. | s-N + s-HS → s-H + s-NS | | 1.0 | 0 | 0 | 1 | 0 | Methodology described in appendix A. |
| 272. | s-N + s-NS → s-S + s-$N_2$ | | 1.0 | 0 | 0 | 1 | 0 | Methodology described in appendix A. |
| 273. | s-N + s-HCS → s-HNCS<br>→ s-HSCN | | 0.5<br>0.5 | 0<br>0 | 0<br>0 | 2<br>2 | 0<br>0 | See Appendix A. |
| 274. | s-NH + s-CS → s-HNCS | | 1.0 | 0 | 1200 | 1 | 600 | Theoretical gas phase value, see appendix A |
| 275. | s-NH + s-HCS → s-NHCHS | | 1.0 | 0 | 0 | 1 | 0 | Methodology described in appendix A. |
| 276. | s-$NH_2$ + s-CS → s-$NH_2CS$ | | 1.0 | 0 | 800 | 3 | 200 | Theoretical gas phase value, see appendix A |
| 277. | s-$NH_2$ + s-HCS → s-$NH_2CHS$ | | 1.0 | 0 | 0 | 1 | 0 | Methodology described in appendix A. |
| 278. | s-O + s-HS → s-HSO | | 1.0 | 0 | 0 | 1 | 0 | Methodology described in appendix A. |
| 279. | s-O + s-SO → s-$SO_2$ | | 1.0 | 0 | 0 | 1 | 0 | Methodology described in appendix A. |
| 280. | s-O + s-HCS → s-H + s-OCS<br>→ s-HS + s-CO | -469<br>-511 | 0.6<br>0.4 | 0<br>0 | 0<br>0 | 2<br>2 | 0<br>0 | From gas phase calculations (Rice et al. 1993, Rice & Chabalowski 1994) considering that OC(H)S, produced by the reaction, will partly isomerize before dissociation. |
| 281. | s-O + s-NS → s-S + s-NO | -174 | 1.0 | 0 | 0 | 1 | 0 | Methodology described in appendix A. |
| 282. | s-S + s-HCO → s-H + s-OCS<br>→ s-HS + s-CO | -246<br>-288 | 0.6<br>0.4 | 0<br>0 | 0<br>0 | 2<br>2 | 0<br>0 | From gas phase calculations (Rice et al. 1993, Rice & Chabalowski 1994) considering that OC(H)S, produced by the reaction, will partly isomerize before dissociation. |
| 283. | s-OH + s-$CH_3SH$→ s-$CH_2SH$ + s-$H_2O$<br>→ s-$CH_3S$ + s-$H_2O$ | | 0<br>1.0 | <br>0 | <br>0 | <br>1.3 | <br>0 | By comparison with the gas phase (Atkinson *et al.* 2004) |


Adams N.G., Smith D., Paulson J.F., 1980, J. Chem. Phys., 72, 288

Adriaens D.A., Goumans T.P.M., Catlow C.R.A., et al., 2010, J. Phys. Chem. C, 114, 1892

Anicich V.G., 2003, JPL Publication 2003, 03-19 NASA.,

Atkinson R., Baulch D.L., Cox R.A., et al., 2004, Atmos. Chem. Phys., 4, 1461

Bauer W., Becker K.H., Meuser R., 1985, Ber. Bunsenges. Phys. Chem., 89, 340

Belau L., Wheeler S.E., Ticknor B.W., et al., 2007, JACS, 129, 10229
Blitz M.A., McKee K.W., Pilling M.J., 2000, Proc. Combust. Inst., 28, 2491
Bradley J.N., Trueman S.P., Whytock D.A., et al., 1973, J. Chem. Soc. Faraday T. 1, 69, 416
Butkovskaya N.I., Setser D.W., 1999, J. Phys. Chem. A, 103, 6921
Cheng B.-M., Eberhard J.r., Chen W.-C., et al., 1997, J. Chem. Phys., 106, 9727
Cupitt L.T., Glass G.P., 1975, Proc. Symp. Chem. Kinet. Data Upper Lower Atmos., 39
Decker B.K., Macdonald R.G., 2001, J. Phys. Chem. A, 105, 6817
Deeyamulla M.P., Husain D., 2006, J. Photochem. Photobiol. A Chem., 184, 347
Dorthe G., Caubet P., Vias T., et al., 1991, J. Phys. Chem., 95, 5109
Ellingson B.A., Truhlar D.G., 2007, JACS, 129, 12765
Eshchenko G., Kacher T., Kerst C., et al., 2002, Chem. Phys. Lett., 356, 181
Ewig F., Rhäsa D., Zellner R., 1987, Berich. Bunsen. Gesell., 91, 708
Fehsenfeld F.C., Ferguson E.E., 1973, J. Geophys. Res., 78, 1699
Fikri M., Meyer S., Roggenbuck J., et al., 2001, Faraday Discuss., 119, 223
Flores J.R., Estévez C.M., Carballeira L., et al., 2001, J. Phys. Chem. A, 105, 4716
Flores J.R., Martinez-Nunez E., Vazquez S.A., et al., 2002, J. Phys. Chem. A, 106, 8811
Galland N., Caralp F., Rayez M.T., et al., 2001, J. Phys. Chem. A, 105, 9893
Geppert W.D., Hamberg M., Thomas R.D., et al., 2006, Faraday Discussions, 133, 177
Gingerich K.A., Finkbeiner H.C., Schmude W.J., 1994, J. Am. Chem. Soc., 116, 3884
Gronowski M., Kolos R., 2014, ApJ, 792, 89
Grotheer H.-H., Rieketr G., Walter D., et al., 1989, Symp. Int. Combust. Proc., 22, 963
Hamberg M., Geppert W.D., Thomas R.D., et al., 2007, Mol. Phys., 105, 899
Hochlaf M., Nicolas C., Poisson L., 2007, J. Chem. Phys., 127
Hunter E.P.L., Lias S.G., 1998, J. Phys. Chem. Ref. Data, 27, 413
Husain D., Ioannou A.X., 1999, J. Photo. Photobio. A, 129, 1
Hynes A.J., Wine P.H., 1987, J. Phys. Chem., 91, 3672
Jourdain J.L., Bras G.L., Combourieu J., 1979, Int. J. Chem. Kinet., 11, 569
Kaminska M., Vigren E., Zhaunerchyk V., et al., 2008, ApJ, 681, 1717
Kerr K.E., Alecu I.M., Thompson K.M., et al., 2015, J. Phys. Chem. A, 119, 7352
Kurylo M.J., Peterson N.C., Braun W., 1971, J. Chem. Phys., 54, 943
Lander D.R., Unfried K.G., Glass G.P., et al., 1990, J. Phys. Chem., 94, 7759
Le Picard S.D., Canosa A., Rowe B.R., et al., 1998, J. Chem. Soc. Faraday T., 94, 2889
Lilenfeld H.V., Richardson R.J., 1977, J. Chem. Phys., 67, 3991
Lin Y.-L., Wang N.-S., Lee Y.-P., 1985, Int. J. Chem. Kinet., 17, 1201

Loison J.-C., Halvick P., Bergeat A., et al., 2012, MNRAS, 421, 1476
Lu C.-W., Wu Y.-J., Lee Y.-P., et al., 2004, J. Chem. Phys., 121, 8271
Maiti B., Schatz G.C., Lendvay G.r., 2004, J. Phys. Chem. A, 108, 8772
Martin D., Jourdain J.L., Le Bras G., 1988, Int. J. Chem. Kinet., 20, 897
Mendes M.B., Buhr H., Berg M., et al., 2012, ApJ, 746, L8
Millar T.J., Adams N.G., Smith D., et al., 1986, MNRAS, 221, 673
Milligan D.B., McEwan M.J., 2000, Chem. Phys. Lett., 319, 482
Montaigne H., Geppert W.D., Semaniak J., et al., 2005, ApJ, 631, 653
Mousavipour S.H., Namdar-Ghanbari M.A., Sadeghian L., 2003, J. Phys. Chem. A, 107, 3752
Nicholas J.E., Amodio C.A., Baker M.J., 1979, J. Chem. Soc. Faraday T., 75, 1868
Nicolas C., Shu J., Peterka D.S., et al., 2005, JACS, 128, 220
Peng J., Hu X., Marshall P., 1999, J. Phys. Chem. A, 103, 5307
Petrie S., 1996, MNRAS, 281, 666
Rice B.M., Cartland H.E., Chabalowski C.F., 1993, Chem. Phys. Lett., 211, 283
Rice B.M., Chabalowski C.F., 1994, J. Phys. Chem., 98, 9488
Ruaud M., Loison J.C., Hickson K.M., et al., 2015, MNRAS, 447, 4004
Scott G.B.I., Milligan D.B., Fairley D.A., et al., 2000, J. Chem. Phys., 112, 4959
Sen A.D., Anicich V., Federman S.R., 1992, ApJ, 391, 141
Shackleford W.L., Mastrup F.N., Kreye W.C., 1972, J. Chem. Phys., 57, 3933
Shannon R.J., Cossou C., Loison J.-C., et al., 2014, RSC Advances, 4, 26342
Smith D., Spanel P., Mayhew C.A., 1992, Int. J. Mass Spectrom., 117, 457
Tiee J.J., Wampler F.B., Oldenborg R.C., et al., 1981, Chem. Phys. Lett., 82, 80
Wakelam V., Loison J.C., Herbst E., et al., 2015, ApJ, Supp. Series, 217, 20
Wakelam V., Smith I.W.M., Herbst E., et al., 2010, Space Sciences Rev., 156, 13
Zhang X., Zou S., Harding L.B., et al., 2004, J. Phys. Chem. A, 108, 8980
